# Supplementary material for: Satori: Towards Proactive AR Assistant with Belief-Desire-Intention User Modeling
Source: arXiv:2410.16668 source file (2025-03-31)
Supplement: Supplementary file 1 [file 01_system.tex]

\newpage
\section{Implementation Details}

\subsection{Backend Streaming Server}
The backend server receives the streaming data from HoloLens 2 headset, processes the data, and sends the processed result back to HoloLens 2. To implement this pipeline, we implement a streaming server with Redis-Stream and create an extension module with the Lambda program. 

\subsubsection{Hardware}
Due to hardware limitations, we are unable to host our entire backend program on a single server. As a result, we distribute the backend server across two devices. One server is equipped with an Intel Core™ i7-8700K CPU @ 3.70GHz and an NVIDIA GeForce GTX 1080 GPU. The other server features an Intel® Core i9-10980XE CPU @ 3.00GHz and two NVIDIA RTX 3090 GPUs.
\begin{table*}[!htbp]
    \centering

\begin{tabular}{|l|p{6cm}|l|}

\hline
Stream                   & Description                                                                                                                   & \multicolumn{1}{c|}{Data Format}    \\ \hline
main                     & The stream which contains the frames sent by HoloLens 2 headset                                                               & \multicolumn{1}{c|}{Image Bytes}    \\ \hline
processed\_main          & The stream which contains the frames processed by an image recognition module to filter out the related frames                & \multicolumn{1}{c|}{Image Bytes}    \\ \hline
guidance                 & The stream used to store the generated guidance result                                                                        & \multicolumn{1}{c|}{JSON}           \\ \hline
assistant:images         & The stream used to store the generated image assistance.                                                                      & \multicolumn{1}{c|}{Protobuf Bytes} \\ \hline
intent:belief            & The stream used to store the inferred belief state.                                                                           & JSON                                \\ \hline
intent:desire            & The stream used to store the inferred desire state                                                                            & JSON                                \\ \hline
intent:task\_plan        & The stream used to store the task plan consisting the desired task plan and action checkpoints generated by the task plan LLM & JSON                                \\ \hline
intent:task:checkpoints  & The stream used to store the inferred states of the action checkpoints                                                        & JSON                                \\ \hline
intent:task:step:nex     & The stream used to store the inferred next intended action.                                                                   & JSON                                \\ \hline
intent:task:step:current & The stream used to store the inferred next intended action.                                                                   & JSON                                \\ \hline
feedback                 & The stream used to store the user' feedback.                                                                                  & JSON                                \\ \hline
\end{tabular}
\caption{The stream list used in the system. We list the stream names, corresponding descriptions, and data formats in the table. The names in the open-sourced code may be slightly different from the names in the development build.}
\label{tab:streams}
\end{table*}

\subsubsection{Redis-Streams Module}
To accommodate this setup and enable data communication across multiple devices, we introduced the Redis-Streams module.
Redis Streams is a feature index designed to handle high-throughput streaming data. It allows for managing time-ordered events and is particularly useful for building message queues and real-time data processing systems. We use it for handling the streaming data generated by HoloLens 2, enabling efficient processing and communication of the data across the HoloLens client, backend server, and distributed model servers.
The basic unit in this module is the \textit{Stream} class, which is defined by a stream key and a pre-defined format, supporting various data types such as the Protobuf bytes, JSON, plain strings, and image bytes. Each stream consists of a series of entries, where each entry represents a piece of data indexed by the timestamp. The stream data can be added, read, and processed by the different clients and servers. We list the streams in Table~\ref{tab:streams}.
Our server supports both WebSocket and HTTP requests, enabling client-side applications to subscribe to streams using WebSocket connections and send new data into the streams via WebSocket as well. This setup provides real-time, bidirectional communication between the HoloLens device and the backend server. For scenarios where WebSocket is not available, we also support data submission and retrieval through standard HTTP requests, offering flexibility in how data is transmitted. 

\subsubsection{Lambda Extension to Redis-Streams Module}
Lambda functions are stateless, event-driven functions that execute in response to specific events or data triggers. In the context of our streaming program, the stateless nature of Lambda functions makes them a suitable choice for handling real-time data processing tasks without the need for persistent state management. Our implementation is based on a class named \textit{Pipeline} (the actual name used in the codebase), which serves as a stateless stream processor. Each Pipeline instance can subscribe to multiple streams, process the data as needed, and publish the processed results to output streams. For example, the object detection module subscribes to image streams, processes the images to detect objects, and then outputs the detected objects in JSON format to another stream.
To simplify the development of such modules, we implemented a set of base classes for tasks such as running GPT models and performing image analysis. These base classes provide common functionalities, allowing other services to extend and implement specific processing logic with minimal effort. Given the high frame rate (fps) of the image stream and the fact that our machine-learning modules may not need or be capable of processing data at such high frequencies, we introduced a frequency adjustment mechanism. This mechanism allows the Lambda function to cache incoming frames and process them at a configurable interval, reducing the computational load and ensuring efficient processing.

\subsection{Client Implementation}
We implemented our HoloLens 2 interface using Unity and the Mixed Reality Toolkit (MRTK). For data communication, we utilized Google’s Protocol Buffers (Protobuf) module and used the NativeWebSocket library to establish WebSocket connections. We acquired the main camera frames from the HoloLens 2 using the Research Mode and the corresponding C++ API.

\subsection{Image assistance generation}
\label{sec:image}
\revision{Generating images in-situ presents challenges as it not only requires understanding the user's interaction context and action but also facilitates a timely generation process that accurately reflects the current task. Following~\cite{DBLP:conf/cvpr/MenonMG24}, image generation must ensure: 1) \textbf{clarity and conciseness}, avoiding unnecessary details that might confuse or overwhelm the user; 2) \textbf{consistent formatting}, as similar design style reduces cognitive load and helps users quickly grasp instructions; 3) \textbf{action-oriented} images that explicitly direct attention and guide the user (with an arrow or indicator) to the target physical objects; and, lastly, 4)  \textbf{coherence} between those objects and the ones in the user's real-world environment.}

When prompting DALL-E 3, the image generation pipeline receives an initial prompt input, which includes the user's next-step action and a list of scene objects. The pipeline then introduces a \textbf{modifier}~\ref{tab:modifiers} using the following template:
\begin{verbatim}
[Object][Attributes][Action].[Indicator][Attributes][Direction].[Background].[Style Modifier].
[Quality Booster]
\end{verbatim}
The prompt template is structured to encapsulate elements of an instructional image in a standardized format. Each element in the prompt template is associated with a specific modifier to refine its description. The basic prompt includes \textit{Object} and \textit{Action} modifiers, which depict the action and the targeted object within the assistance image. The \textit{Attribute} modifier incorporates real-world attributes such as color, shape, and materials of the objects, enhancing task immersion and operational accuracy. Additionally, \textit{Indicator} modifiers, such as arrows, and \textit{Direction} modifiers explicitly highlight the action direction or focal points for user attention. The \textit{Background} modifier removes unnecessary details, clarifying the image. The \textit{Style Modifier} governs the aesthetic of the image; we choose to apply the ``flat, instructional illustration'' style based on feedback from experiments, ensuring that the visuals maintain a consistent appearance. Lastly, the \textit{Quality Booster} enhances image quality with descriptors such as ``accurate'' and ``concise,'' further ensuring clarity and effectiveness in the visual assistance provided.

For generating multiple images to support complex actions in the forms of animation, we use a similar template and pipeline as described above in sub-steps (generated by the task planner) and create one image per sub-step, sending it to the DALL-E 3 model in parallel.

\begin{table}[]
\begin{tabular}{lll}
\toprule
Modifier        & Description                                                                        & Example                    \\ \midrule
Object          & Denotes the main object or the tool & button                     \\
Indicator       & Graphic element that points out specific parts or directions     & arrow                      \\
Attribute       & Attributes of objects or indicators, such as shape and color                       & red                        \\
Action          & Specifies the action being performed by the object                                 & press                      \\
Direction       & Clarifies the direction in which the action or attention is guided        & pointing to right          \\
Background      & Specifies the absence or presence of a background                                  & no background              \\
Style Modifier  & Dictates the artistic style of the illustration                                    & instructional illustration \\
Quality Booster & Enhancements that improve the overall clarity and effectiveness       & accuracy                   \\ \bottomrule
\end{tabular}
\caption{Taxonomy of image assistance generation prompt modifiers.} 
\label{tab:modifiers} 
\end{table}
