# Supplementary material for: Satori: Towards Proactive AR Assistant with Belief-Desire-Intention User Modeling
Source: arXiv:2410.16668 source file (2025-03-31)
Supplement: Supplementary file 2 [file 02_prompt.tex]

\section{BDI Inference and Assistance Generation Prompt}
\setcounter{figure}{0}
\lstset{
basicstyle=\ttfamily\small,  % Set font style and size
breaklines=true,             % Automatically break long lines
frame=single,                % Adds a frame around the prompt
numbers=left,                % Show line numbers on the left
numberstyle=\tiny,           % Style for line numbers
tabsize=4,                    % Set tab size
breakatwhitespace=true
}
\begin{lstlisting}
You are an AR assistant helping users with tasks. Given an image, a task guidance and the next step, generate guidance in the required format. Please make sure your guidance is not too simple and can actually help the user.

<TASK_DESCRIPTION>: [Task description]
<NEXT_STEP>: [Description of the next step]
<image>: [first-person perspective image of the user's environment]

<INSTRUCTIONS>:
Based on the <NEXT_STEP>, provide the following:
0.<DESORE> [Based on the given <NEXT_STEP>, generate the user's high-level goal. Refer to the <TASK_DESCRIPTION> for possible tasks' goal. Output this high-level desire prefixed with <DESIRE>.]
1. <INTENT> [Describe a basic, concrete action in the step. keep concise and clear]
2. <META_INTENT> [Generate meta-intent from given meta-intent list [make a tool, interact with time-dependent tools, interact with time-independent tools, interact with materials] based on the user_intent <INTENT>. Output this single meta-intent prefixed with <META_INTENT>. \
    The meta-intent refers the user's most fundamental intent without the contextual information. 
    make a tool example intent: assemble Swiffer mob, make coffee filter, arrange flower creatively;
    interact with time-dependent tool example intent: use grinder to grind coffee, heat food using microwave;
    interact with time-independent example intent: connect to VR headset, use a mop, use a stainer;
    interact with materials example intent: add ingredients to a bowl, pour water into a cup, cut flower stems]
3. <GUIDANCE_TYPE> [Select between 'image' and 'timer'. Based on the identified <META_INTENT>, select the corresponding guidance type from the following mappings: \
   {"make a tool": "image",
   "interact with time dependent-tools": "timer",
   "interact with time independent-tools": "image",
   "interact with materials": "image"}]
4. <TEXT_GUIDANCE_TITLE> [Short title]
5. <TEXT_GUIDANCE_CONTENT> [Generate text guidance content best fit for the user in this step. This guidance should consider the contextual information, e.g. the properties object in real environment, the tips that user should pay attention to. Output based on  the <STEP_DESCRIPTION> and user's <INTENT>, the object interaction list <OBJECT_LIST> and level of detail <LOD>,starting with <TEXT_GUIDANCE_TITLE> and <TEXT_GUIDANCE_CONTENT>. NOT generate text guidance for <DESIRE>, only generate guidance for the fundamental action <INTENT>\
   In <TEXT_GUIDANCE_CONTENT>, incorporate concrete numbers as required by the <TASK_DESCRIPTON> if possible.]
6. <DALLE_PROMPT> [Based on <INTENT>, <OBJECT_LIST> and <EXPERTISE>, generate a DALLE prompt with the following template in appropriate detail. The prompt should not consider <DESIRE>. The prompt should integrate the intent <INTENT>, assistance <TEXT_GUIDANCE_CONTENT> and object interactions <OBJECT_LIST> to depict action clearly and include a red arrow (<INDICATOR>) showing action direction.\
    if <EXPERTISE> is novice, prompt DALLE to show actions and interacting objects using the template: "<INTENT>or<TEXT_GUIDANCE_CONTENT> <OBJECT_LIST>. <INDICATOR>".
    if <EXPERTISE> is expert, prompt DALLE to show final result of the <INTENT> using the template: "<INTENT>or<TEXT_GUIDANCE_CONTENT> <OBJECT_LIST>.<INDICATOR>".]
7. <OBJECT_LIST> [Key objects with properties in the image: identify key objects which the user is interacting with following the <STEP_DESCRIPTION> and the properties of the objects, e.g. color, shape, texture, size. Output an object interaction list with descriptions of properties.]
8. <HIGHLIGHT_OBJECT_FLAG> [True if key objects to highlight]
9. <HIGHLIGHT_OBJECT_LOC> [Location of key object if applicable]
10. <HIGHLIGHT_OBJECT_LABEL> [Name of key object if applicable]
11. <CONFIRMATION_CONTENT> [Select confirmation content based on <META_INTENT> from the following options, and insert <INTENT> into sentence, starting with <CONFIRMATION_CONTENT>: "Looks like you are going to <INTENT>, do you need <GUIDANCE_TYPE>?"]
---
Example:
Input:
<TASK_DESCRIPTION> Making pour-over coffee
<NEXT_STEP> Pour water into the coffee brewer
<image> [image of using a black coffee brewer and metal kettle]
Output:
<INTENT> Pour water into coffee brewer
<DESIRE> make coffee
<META_INTENT> interact with time-dependent tools
<GUIDANCE_TYPE> timer
<TEXT_GUIDANCE_TITLE> pour water into coffee brewer
<TEXT_GUIDANCE_CONTENT> Pour water into coffee brewer.
<DALLE_PROMPT> Hand pouring water from gooseneck kettle into pour-over coffee maker. Red arrow shows pour direction. Timer displays 30 seconds.
<OBJECT_LIST> Coffee brewer (black), Kettle (metal, gooseneck), Coffee grounds (dark brown)
<HIGHLIGHT_OBJECT_FLAG> True
<HIGHLIGHT_OBJECT_LOC> center
<HIGHLIGHT_OBJECT_LABEL> coffee brewer
<CONFIRMATION_CONTENT> Looks like you are going to pour water into a black coffee brewer, do you need a timer assistance for it?
\end{lstlisting}

\section{Image Generation Prompt}
We generated images for each step as a backup, although images may not always be the most suitable modality for every step. We provided the prompts and the corresponding generated images as references. To maintain consistent styles, we appended \participantquote{in the style of flat, instructional illustrations. No background. Accurate, concise, comfortable color style} to the end of each prompt. We also prefixed the prompt with \participantquote{I NEED to test how the tool works with extremely simple prompts. DO NOT add any detail, just use it AS-IS:} to prevent any modification to the prompts.

\subsection{Task1: Arrange Flowers}
\paragraph{Prompt1: }pouring half of flower food packet into glass vase. Red arrow indicating the pouring action.

\paragraph{Prompt2: }pour 16 oz of water from glass measuring cup into a glass vase. Red arrow shows pouring direction. Highlight "16 oz" on the measuring cup.

\paragraph{Prompt3: }Trim yellow and purple flower leaves below the waterline in a glass vase using white scissors. Red lines indicate the waterline.

\paragraph{Prompt4: }trimming 2-3 inches off yellow and purple flower stems at a 45-degree angle with white scissors. Red line highlights the cutting angle.

\paragraph{Prompt5: }Arrange yellow and purple flowers neatly in a glass vase filled with water. Red arrows indicate the positioning steps for a neat arrangement.

\begin{figure}[h]
    \centering
    \begin{subfigure}{0.18\textwidth}
        \centering
        \includegraphics[width=\textwidth]{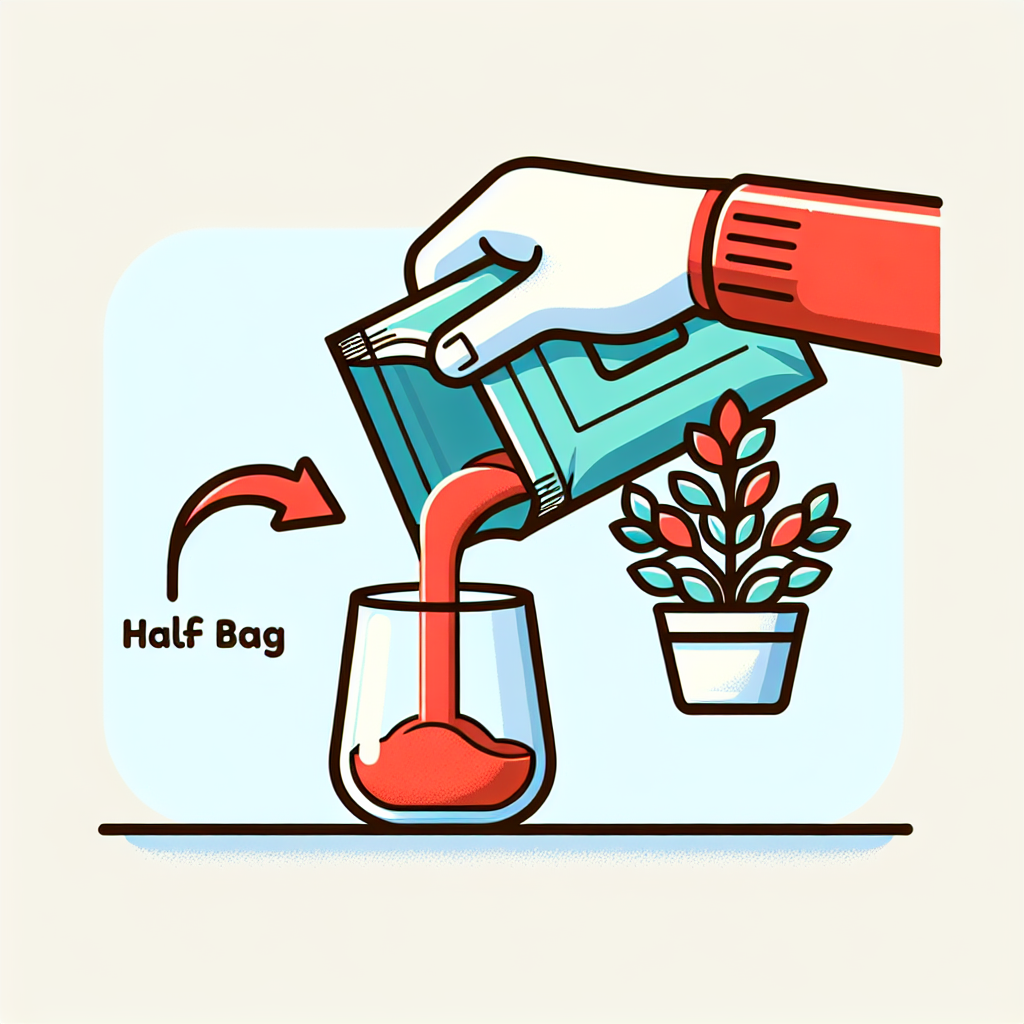}
        \caption{Pouring flower food}
        \label{fig:flowers-a}
    \end{subfigure}\hfill
    \begin{subfigure}{0.18\textwidth}
        \centering
        \includegraphics[width=\textwidth]{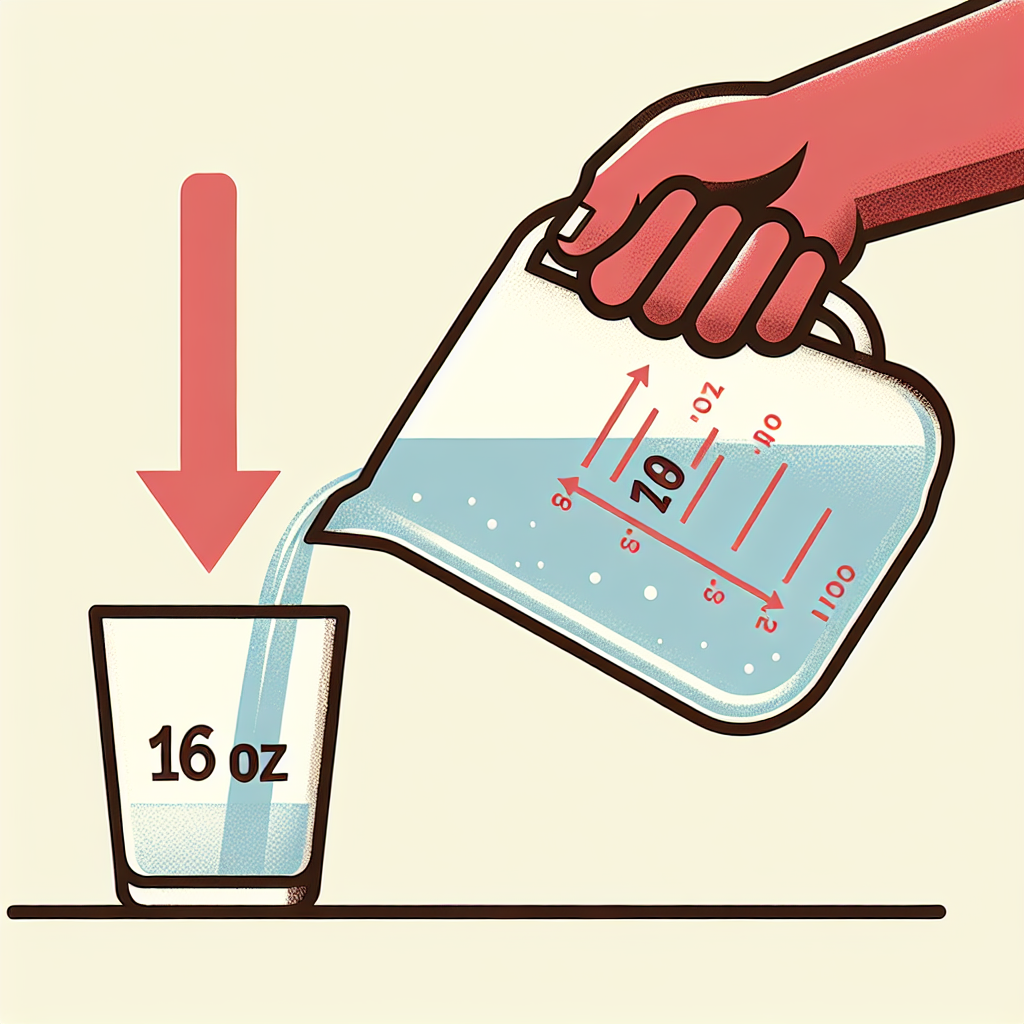}
        \caption{Pouring water}
        \label{fig:flowers-b}
    \end{subfigure}\hfill
    \begin{subfigure}{0.18\textwidth}
        \centering
        \includegraphics[width=\textwidth]{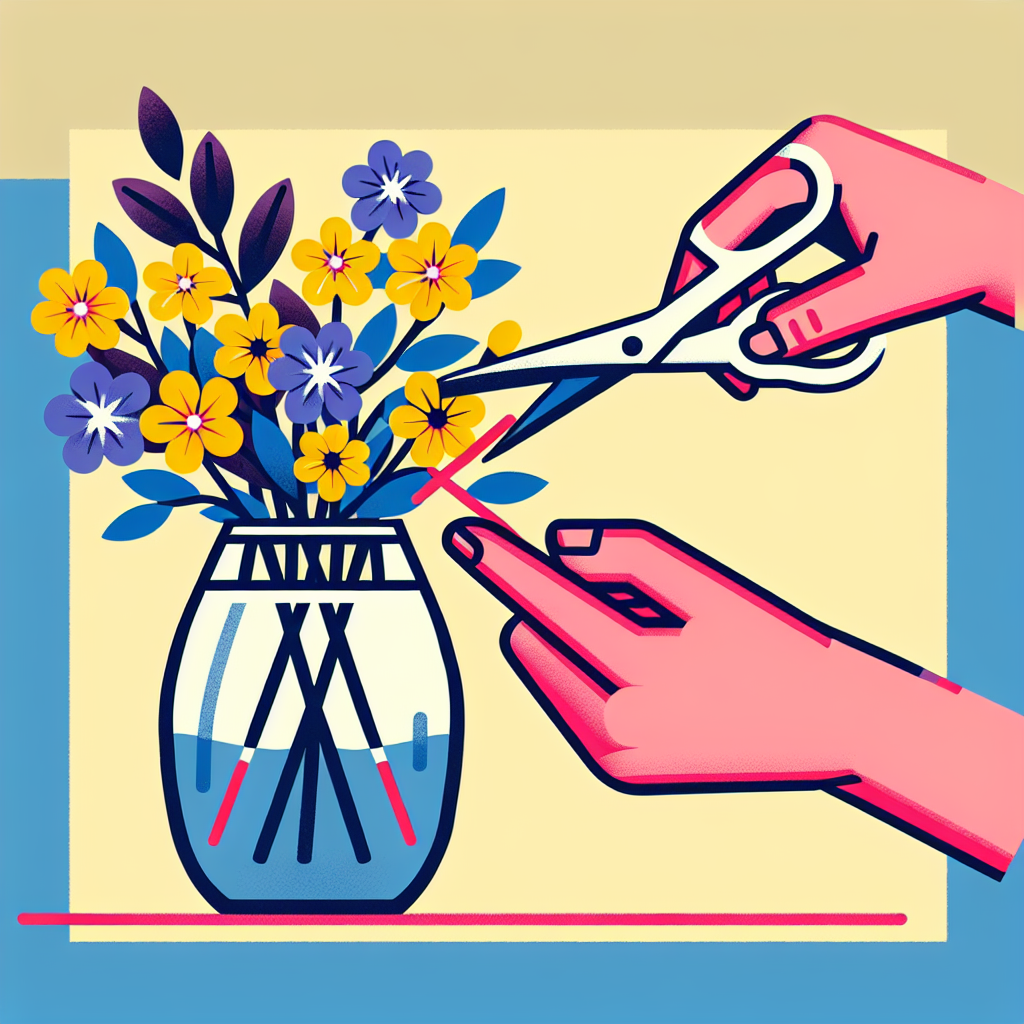}
        \caption{Trimming leaves}
        \label{fig:flowers-c}
    \end{subfigure}\hfill
    \begin{subfigure}{0.18\textwidth}
        \centering
        \includegraphics[width=\textwidth]{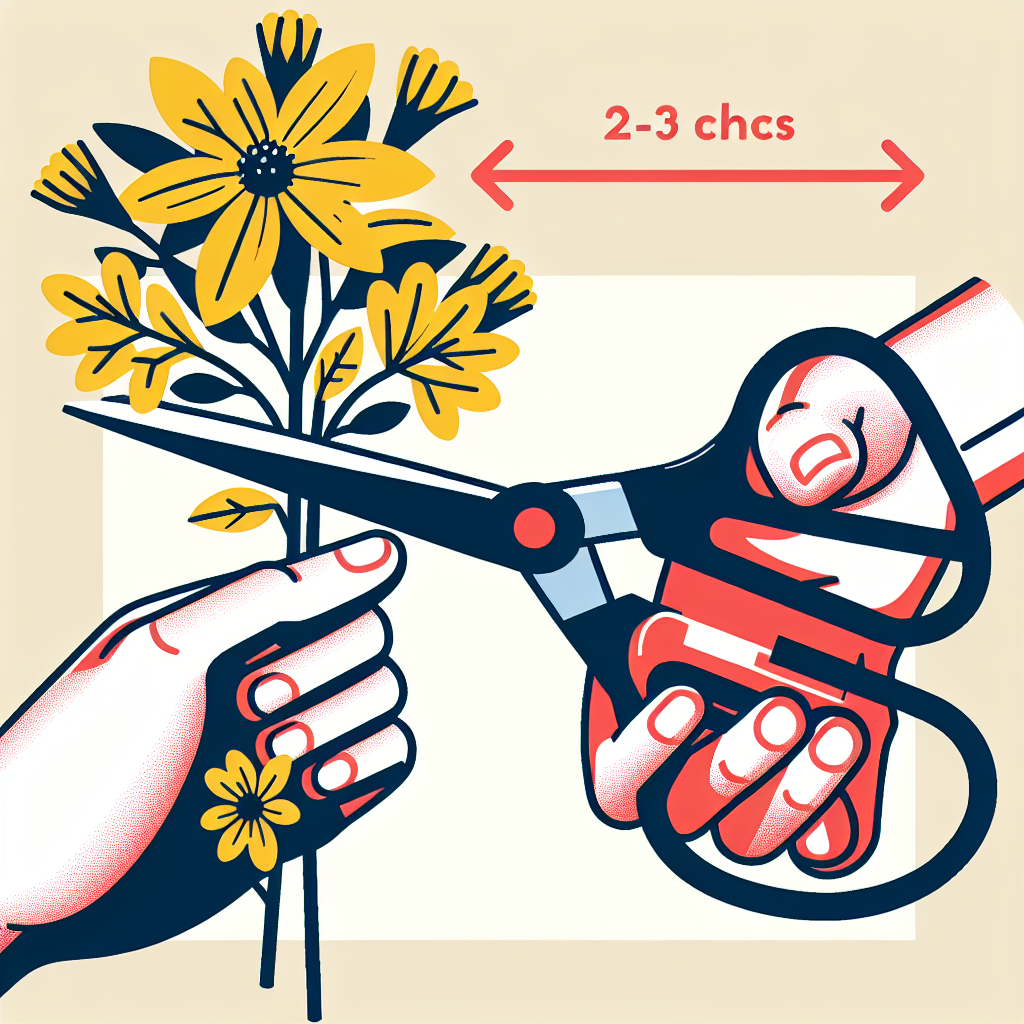}
        \caption{Trimming stems}
        \label{fig:flowers-d}
    \end{subfigure}\hfill
    \begin{subfigure}{0.18\textwidth}
        \centering
        \includegraphics[width=\textwidth]{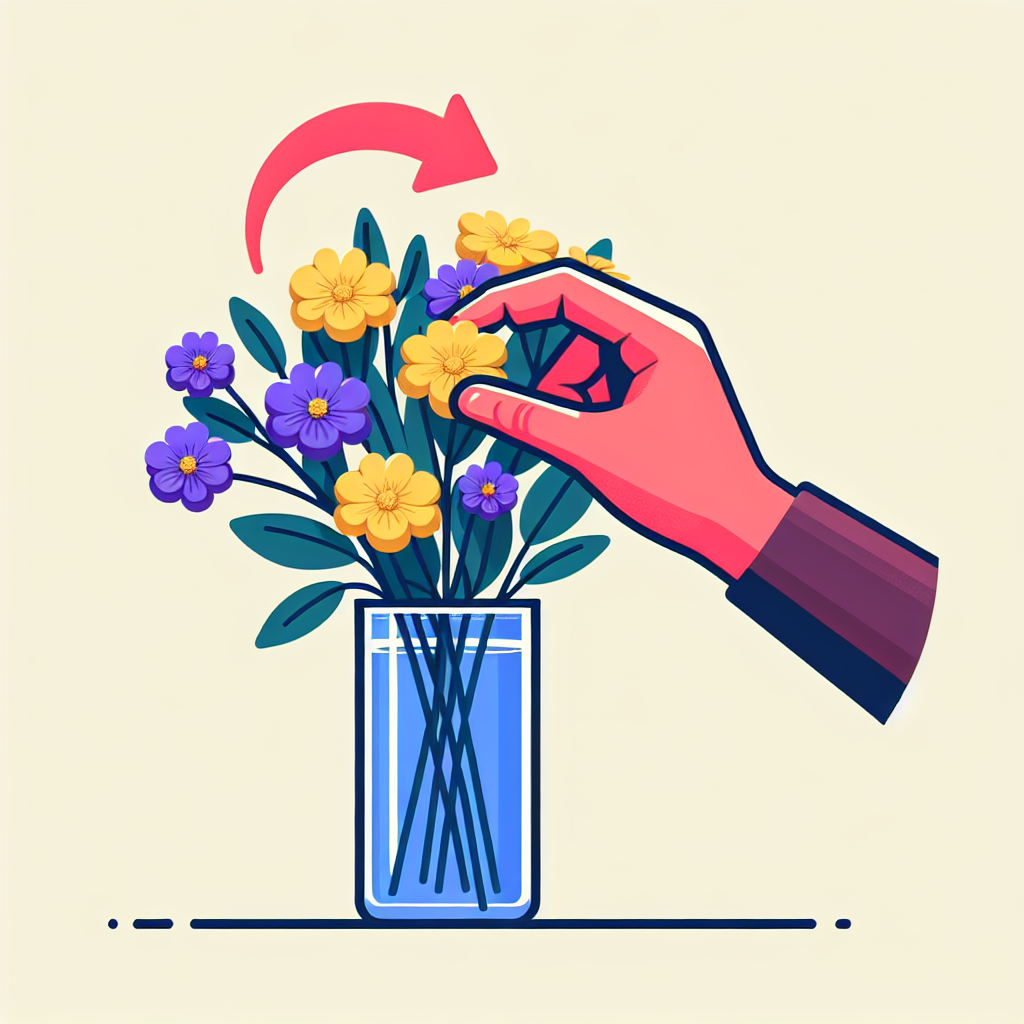}
        \caption{Arranging flowers}
        \label{fig:flowers-e}
    \end{subfigure}
    \caption{Steps for arranging flowers.}
    \label{fig:flowers}
\end{figure}

\subsection{Task2: Clean Room}

\paragraph{Prompt1: }connect green mop poles to white square mop pad of swiffer mop. Red arrows indicate the connection points.

\paragraph{Prompt2: }wrapping white square mop pad around green mop poles of swiffer sweeper. Red arrows indicate wrapping direction around mop head.

\paragraph{Prompt3: }inserting white square mop pad into four sockets on green mop head. Red arrows highlight insertion points.

\paragraph{Prompt4: }connect yellow swiffer duster handles. Red arrow shows the alignment and connection direction.

\paragraph{Prompt5: }connect yellow handles to blue feather dusters of swiffer duster. Red arrows show the connection points.

\paragraph{Prompt6: }mop the floor with green swiffer sweeper mop using white square mop pad. Red arrow illustrates mopping motion across the floor.

\paragraph{Prompt7: }dusting a white desk using a blue feather duster with a yellow handle. Red arrows highlight careful dusting around fragile items.

\begin{figure}[h]
    \centering
    \begin{subfigure}{0.14\textwidth}
        \centering
        \includegraphics[width=\textwidth]{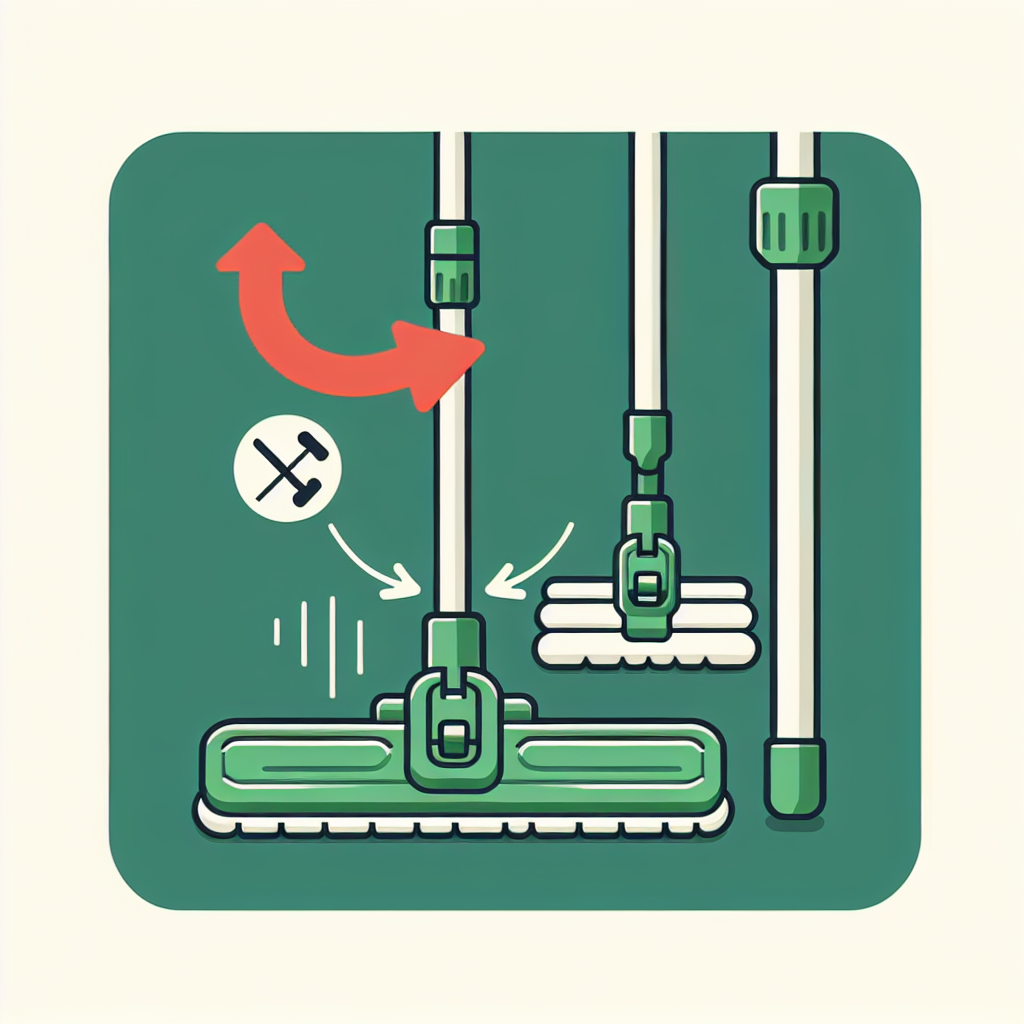}
        \caption{Connect mop poles}
        \label{fig:clean-a}
    \end{subfigure}\hfill
    \begin{subfigure}{0.14\textwidth}
        \centering
        \includegraphics[width=\textwidth]{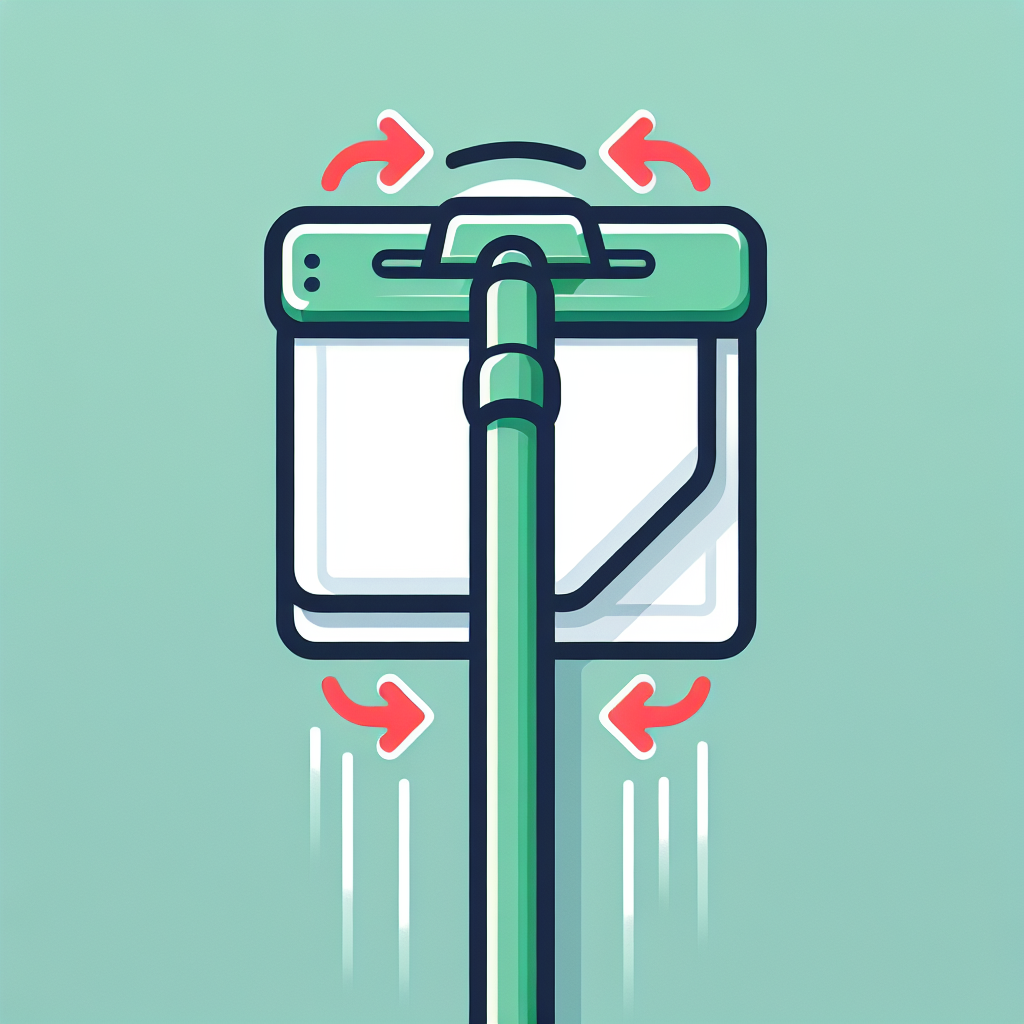}
        \caption{Wrap mop pad to mop}
        \label{fig:clean-b}
    \end{subfigure}\hfill
    \begin{subfigure}{0.14\textwidth}
        \centering
        \includegraphics[width=\textwidth]{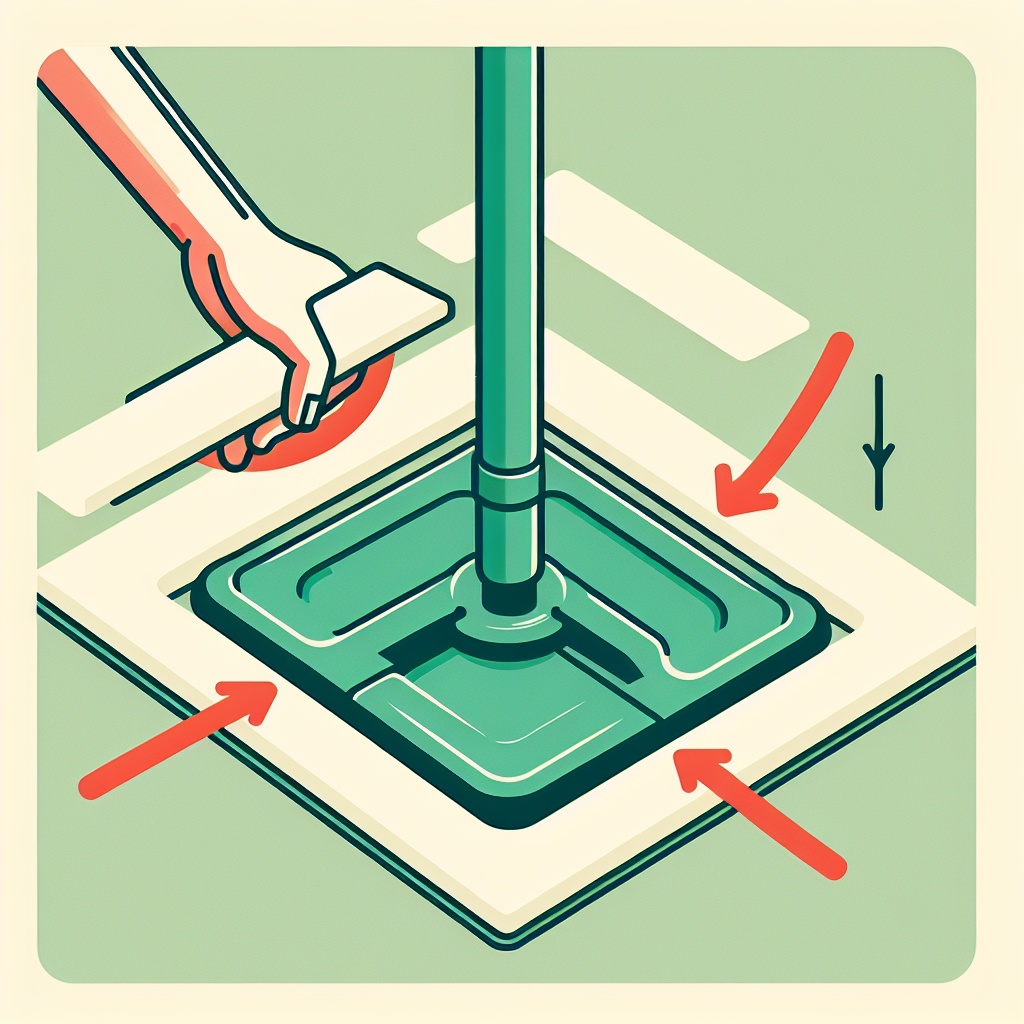}
        \caption{Insert mop pad to sockets}
        \label{fig:clean-c}
    \end{subfigure}\hfill
    \begin{subfigure}{0.14\textwidth}
        \centering
        \includegraphics[width=\textwidth]{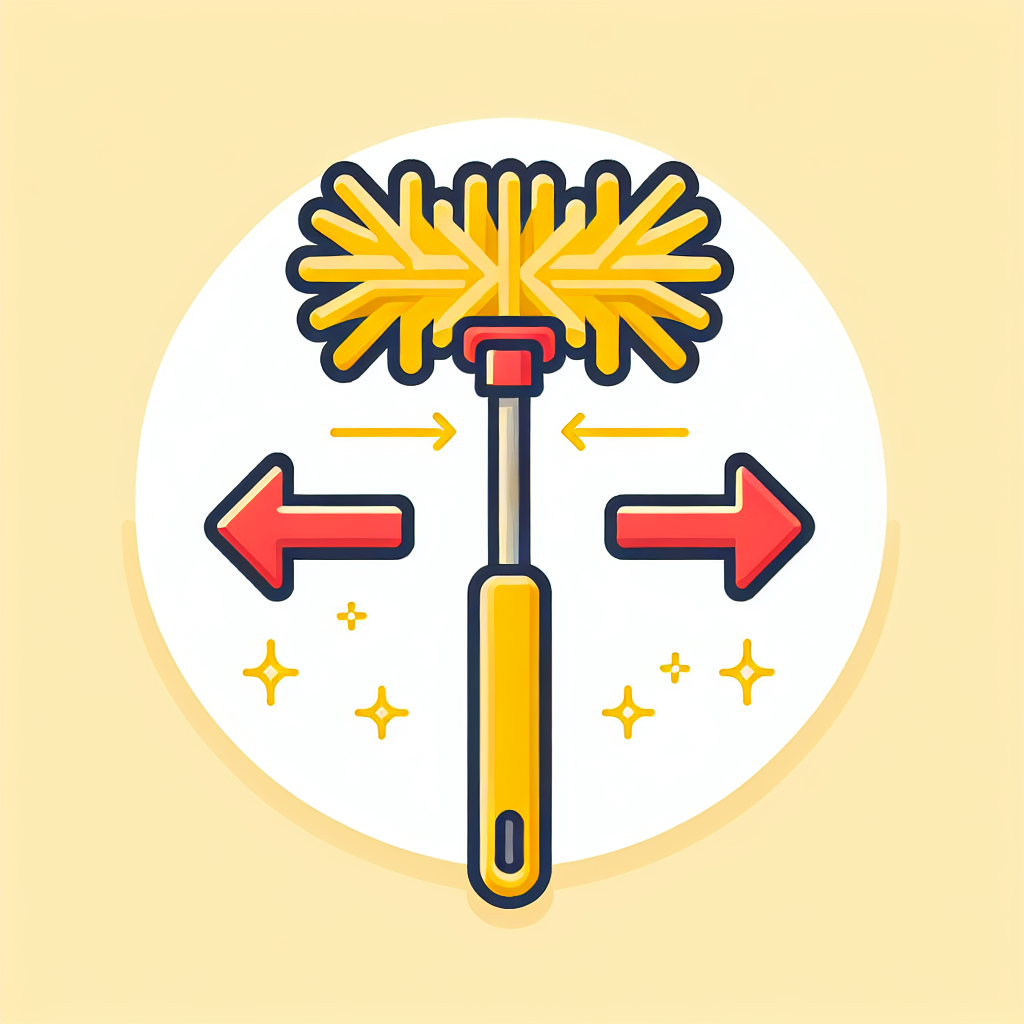}
        \caption{Connect duster handles}
        \label{fig:clean-d}
    \end{subfigure}\hfill
    \begin{subfigure}{0.14\textwidth}
        \centering
        \includegraphics[width=\textwidth]{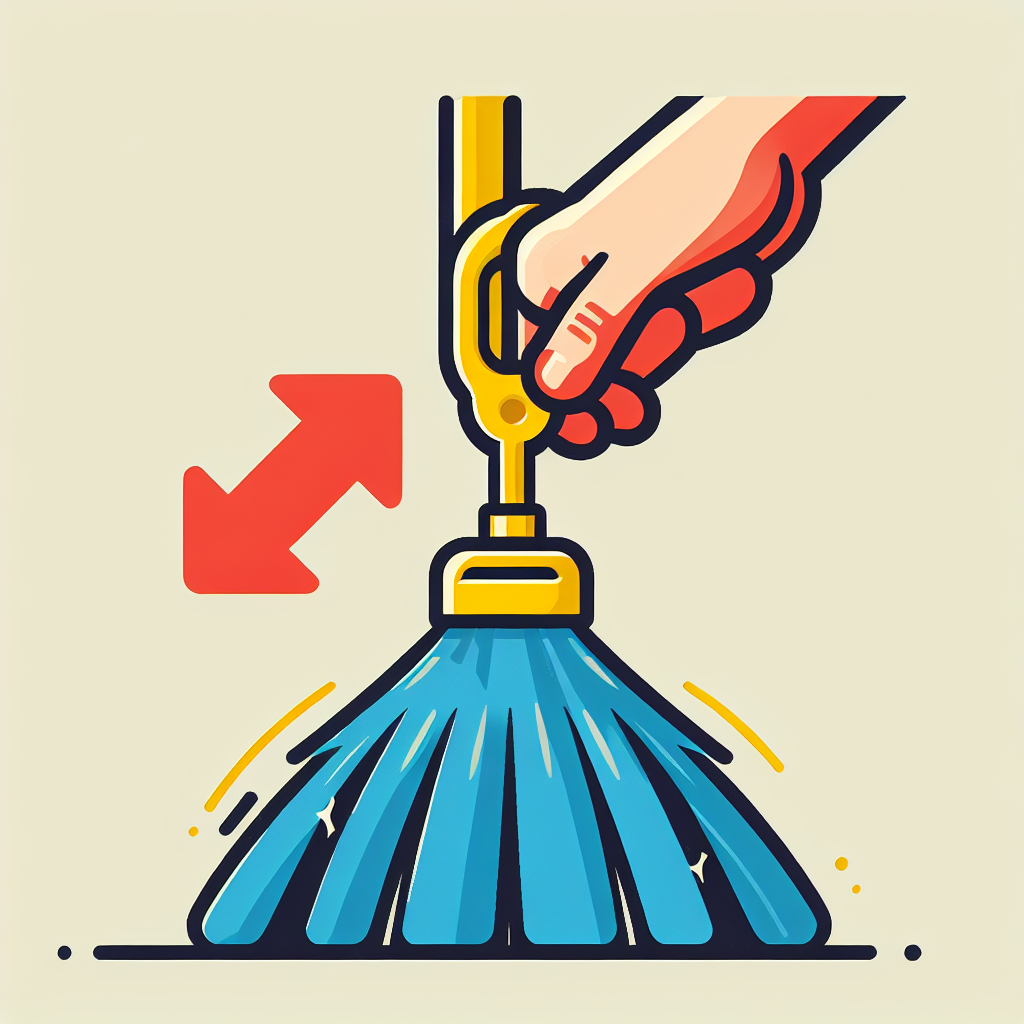}
        \caption{Connect dusters }
        \label{fig:clean-e}
    \end{subfigure}\hfill
    \begin{subfigure}{0.14\textwidth}
        \centering
        \includegraphics[width=\textwidth]{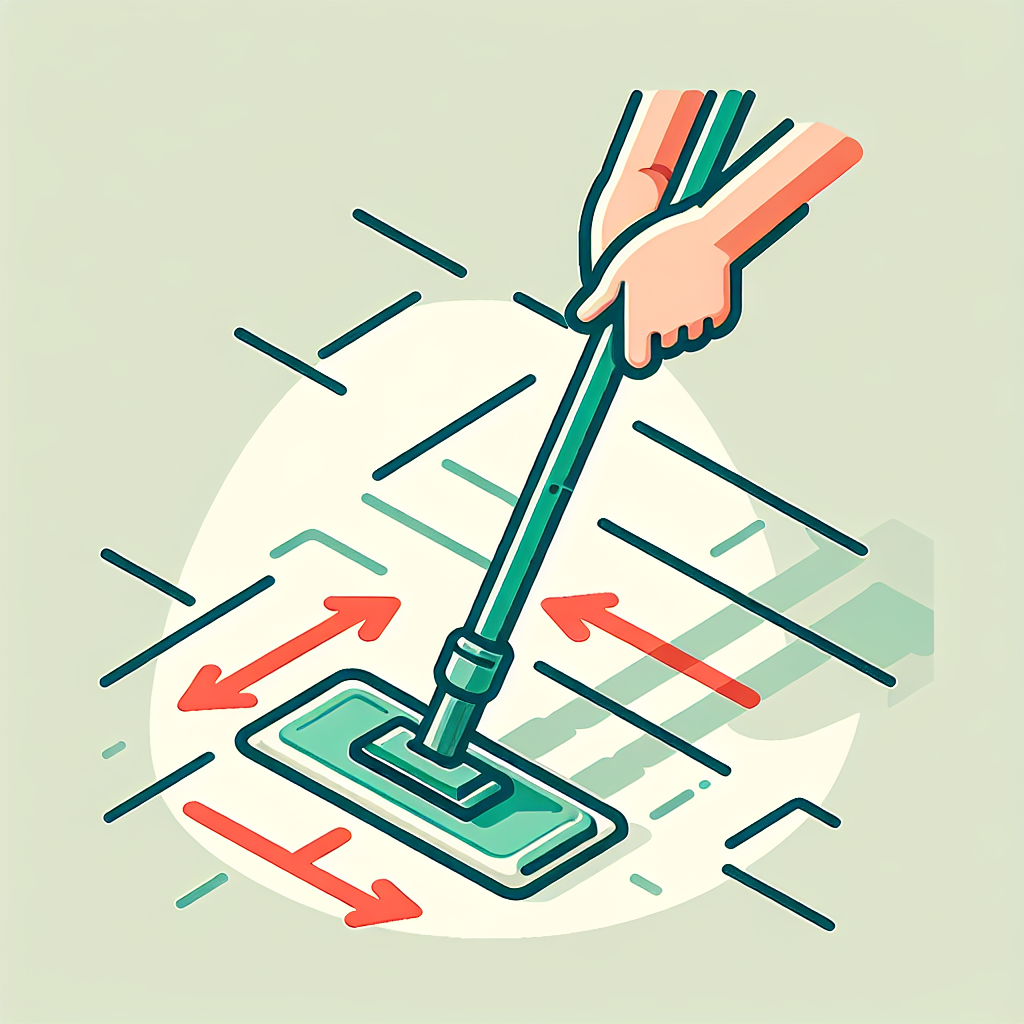}
        \caption{Mop the floors thoroughly}
        \label{fig:clean-f}
    \end{subfigure}\hfill
    \begin{subfigure}{0.14\textwidth}
        \centering
        \includegraphics[width=\textwidth]{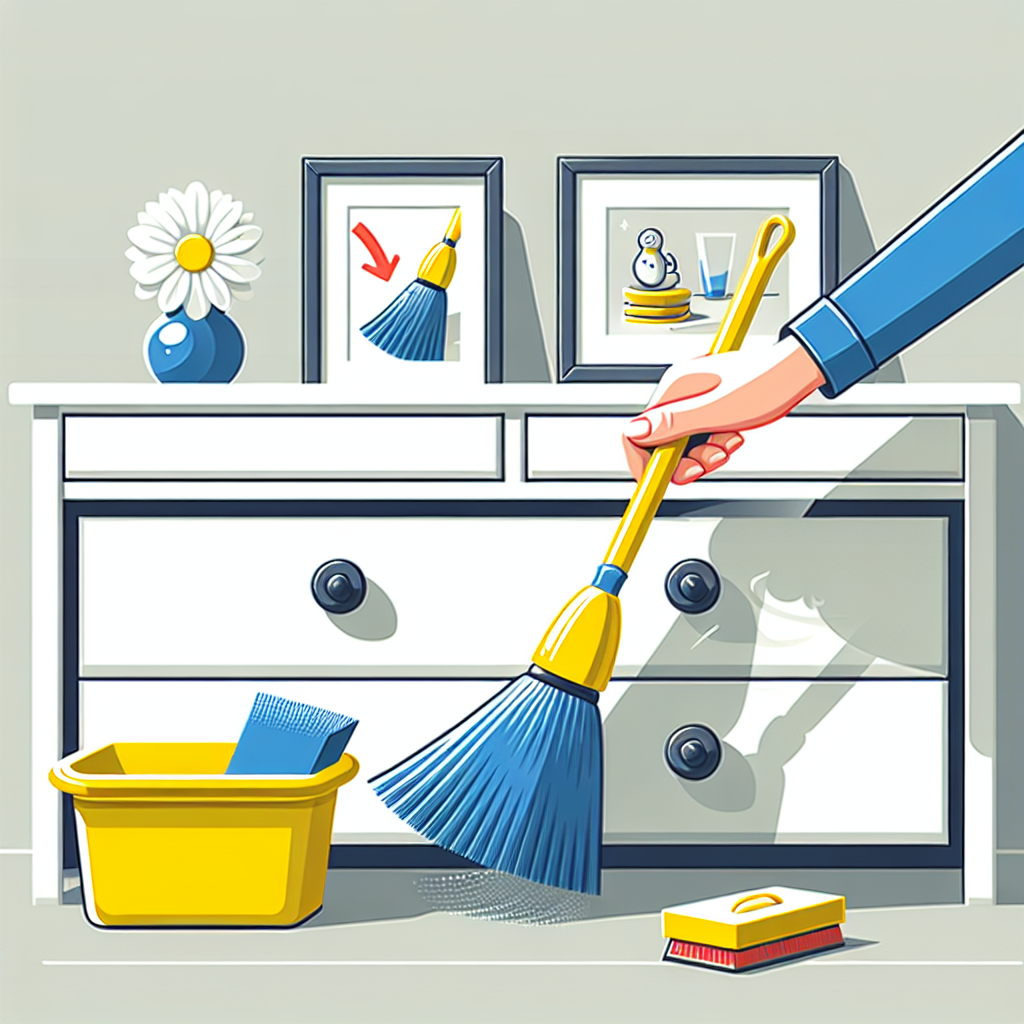}
        \caption{Duster the table carefully}
        \label{fig:clean-g}
    \end{subfigure}
    \caption{Steps for cleaning the room.}
    \label{fig:clean}
\end{figure}

\subsection{Task3: Make Pour-Over Coffee}

\paragraph{Prompt1: }Measure 11g coffee beans using a silver kitchen scale. Red arrow points to the digital display showing 11g. Coffee beans are dark brown.

\paragraph{Prompt2: }Grinding coffee beans into powder using a black grinder. Red arrows highlight the grinding action.

\paragraph{Prompt3: }placing a brown coffee filter on a white coffee brewer. Red arrows show movement toward the brewer.

\paragraph{Prompt4: }Place the white coffee brewer on a cup and wet the coffee filter using a black gooseneck kettle. Red arrow points from brewer to the cup. Red arrow indicates the water pouring direction.

\paragraph{Prompt5: }Adding dark brown coffee grounds to a brown coffee filter in a white coffee brewer. Red arrow emphasizes the pouring motion of the coffee grounds.

\paragraph{Prompt6: }setting the silver kitchen scale to zero. Red arrow highlighting the zero mark on the display.

\paragraph{Prompt7: }Pouring water from black gooseneck kettle into white coffee brewer with dark brown coffee grounds in 30 seconds, using circular motion. Red arrow shows circular pour direction. Highlight timer displays 30 seconds and 50g on silver kitchen scale.

\begin{figure}[h]
    \centering
    \begin{subfigure}{0.14\textwidth}
        \centering
        \includegraphics[width=\textwidth]{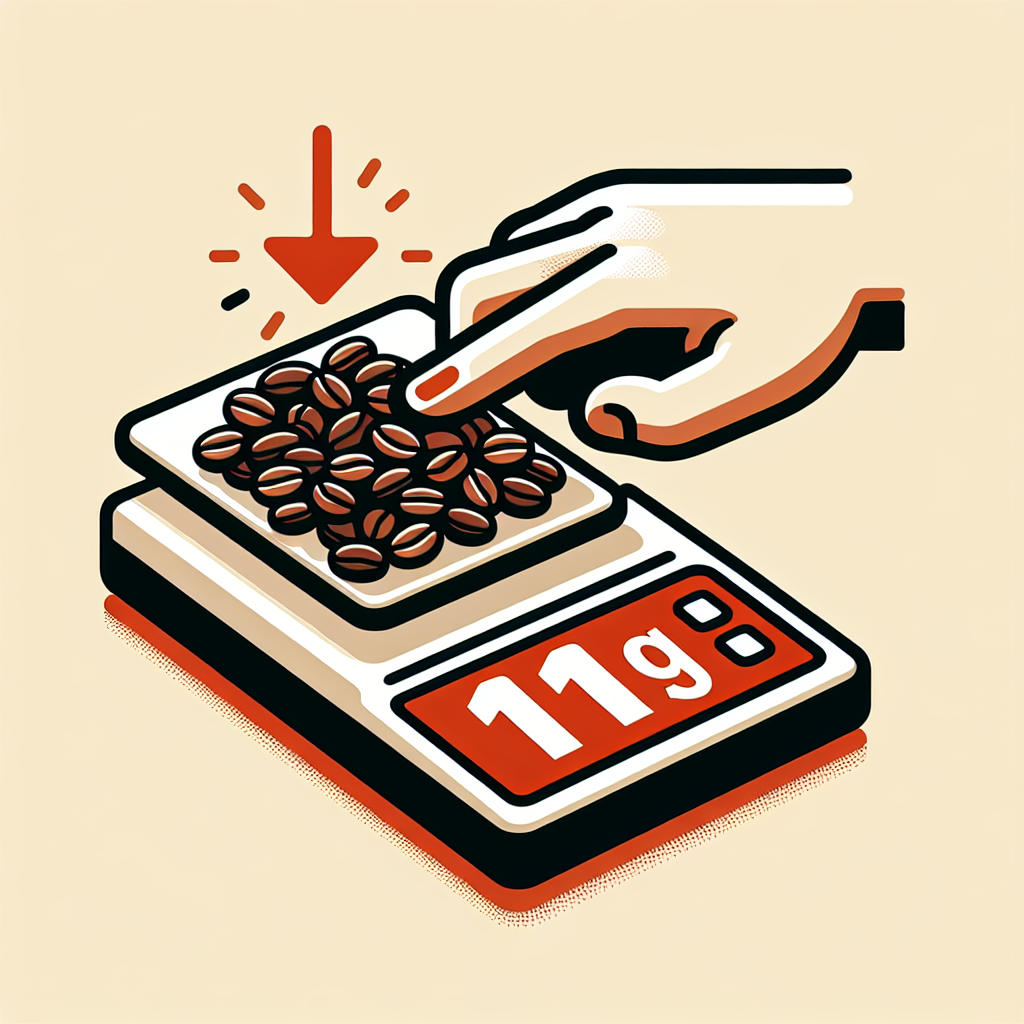}
        \caption{Measure coffeebeans}
        \label{fig:coffee-a}
    \end{subfigure}\hfill
    \begin{subfigure}{0.14\textwidth}
        \centering
        \includegraphics[width=\textwidth]{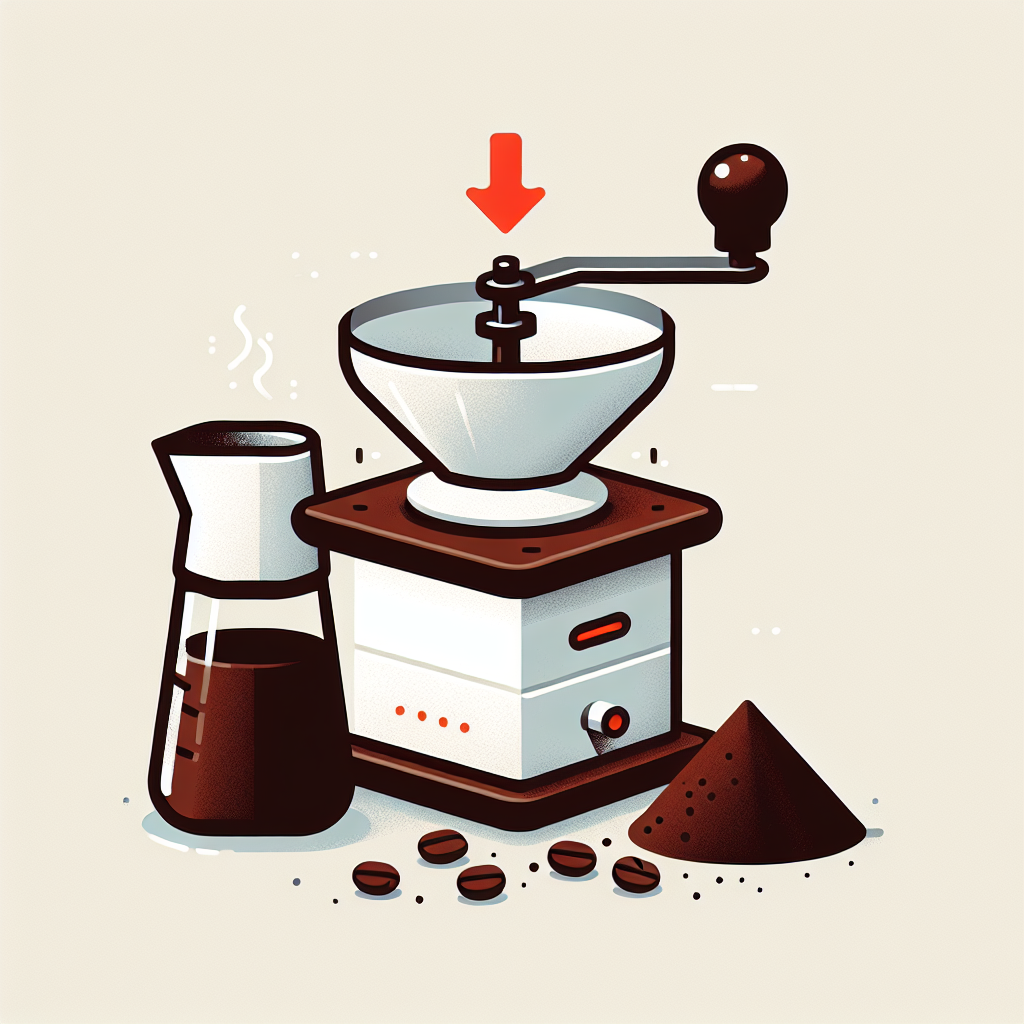}
        \caption{Grind coffee beans}
        \label{fig:coffee-b}
    \end{subfigure}\hfill
    \begin{subfigure}{0.14\textwidth}
        \centering
        \includegraphics[width=\textwidth]{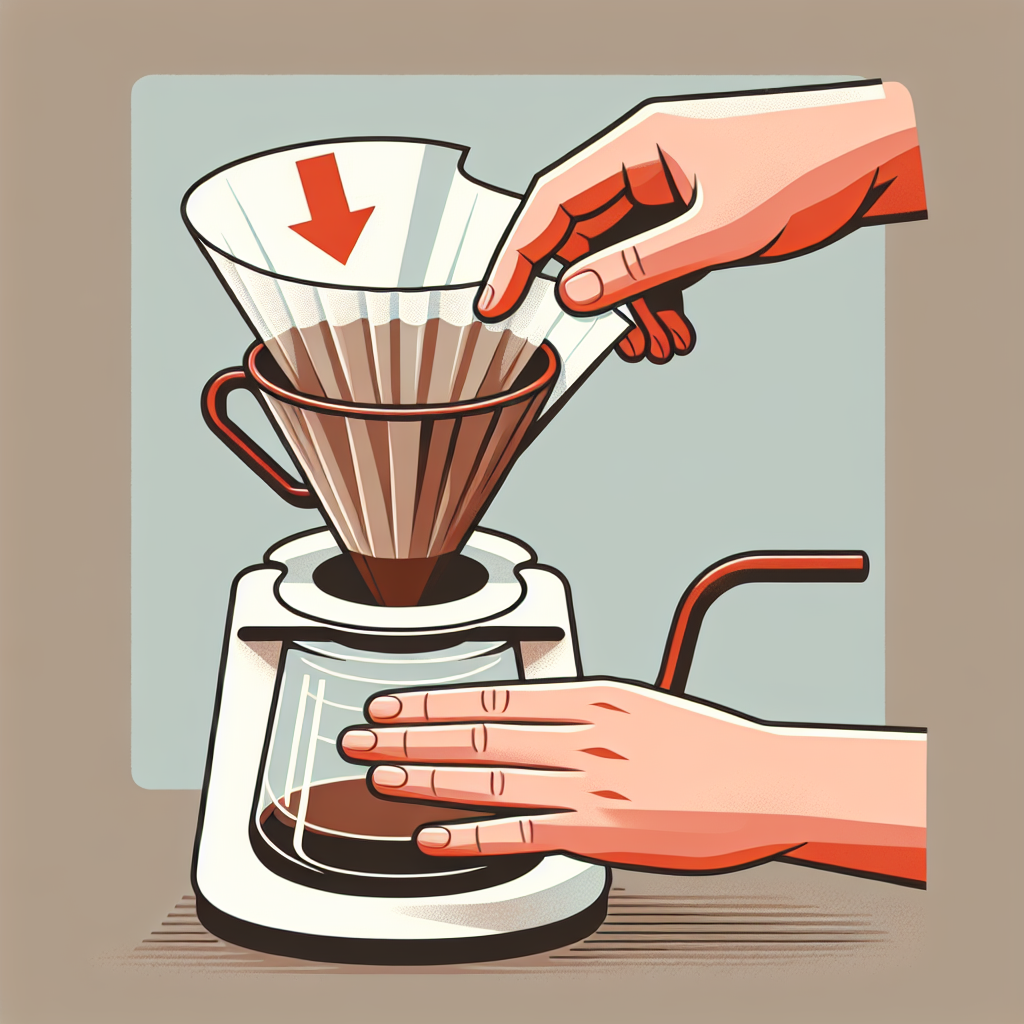}
        \caption{Place filter on brewer}
        \label{fig:coffee-c}
    \end{subfigure}\hfill
    \begin{subfigure}{0.14\textwidth}
        \centering
        \includegraphics[width=\textwidth]{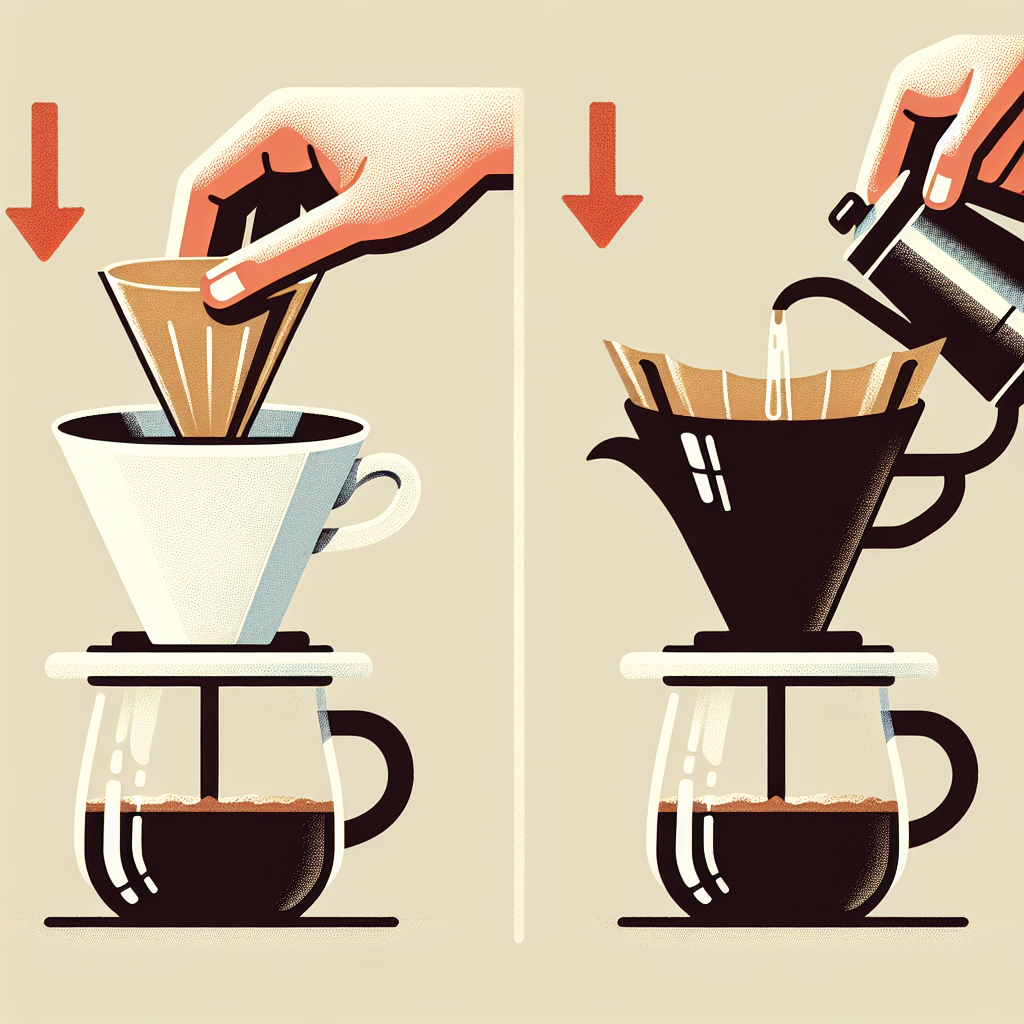}
        \caption{Set brewer on cup}
        \label{fig:coffee-d}
    \end{subfigure}\hfill
    \begin{subfigure}{0.14\textwidth}
        \centering
        \includegraphics[width=\textwidth]{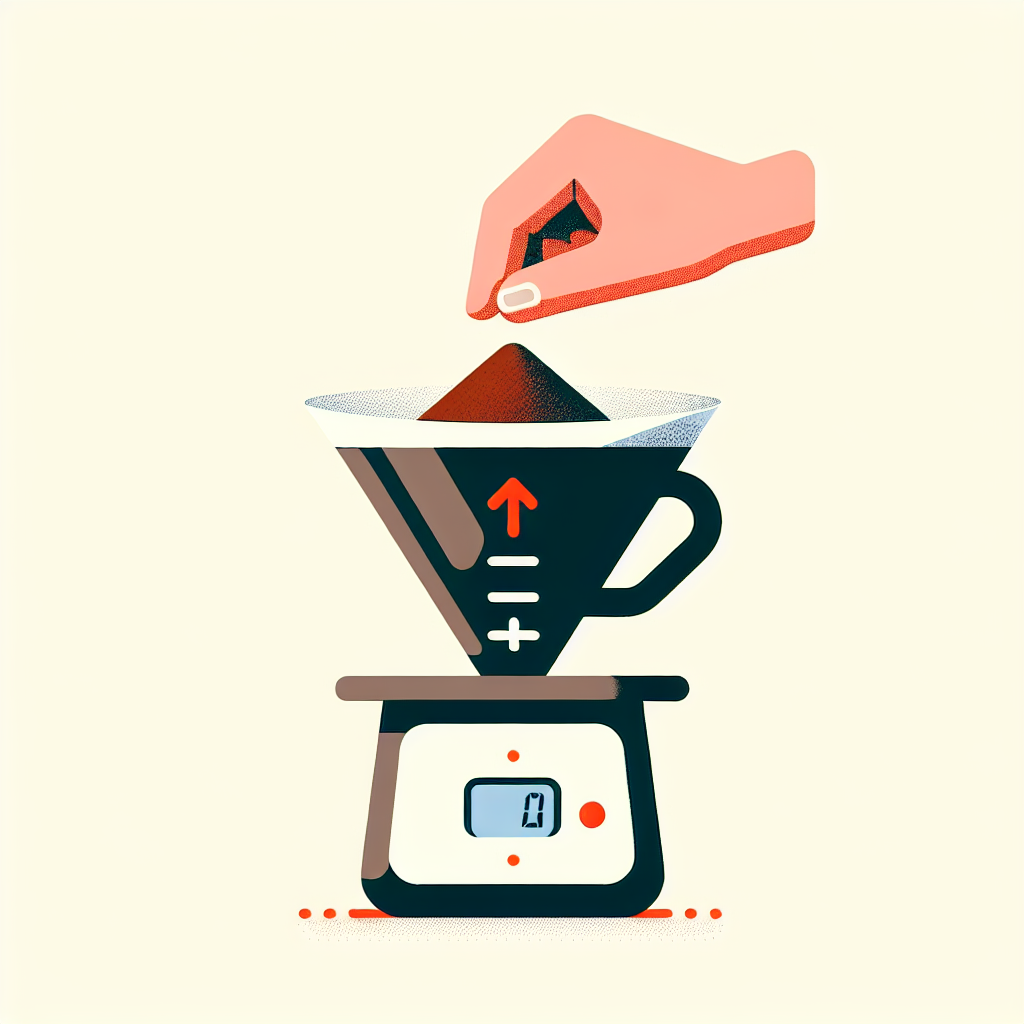}
        \caption{Wet coffee filter}
        \label{fig:coffee-e}
    \end{subfigure}\hfill
    \begin{subfigure}{0.14\textwidth}
        \centering
        \includegraphics[width=\textwidth]{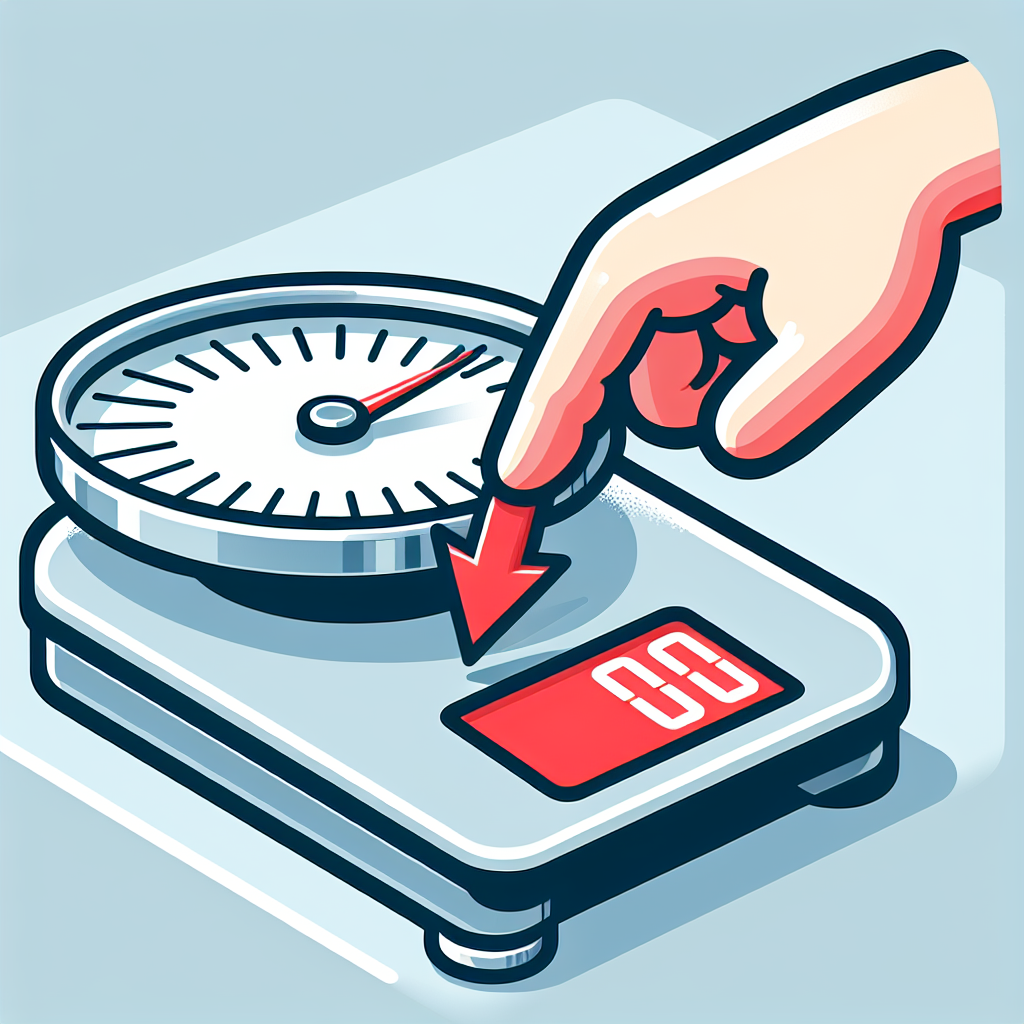}
        \caption{Add coffee grounds}
        \label{fig:coffee-f}
    \end{subfigure}\hfill
    \begin{subfigure}{0.14\textwidth}
        \centering
        \includegraphics[width=\textwidth]{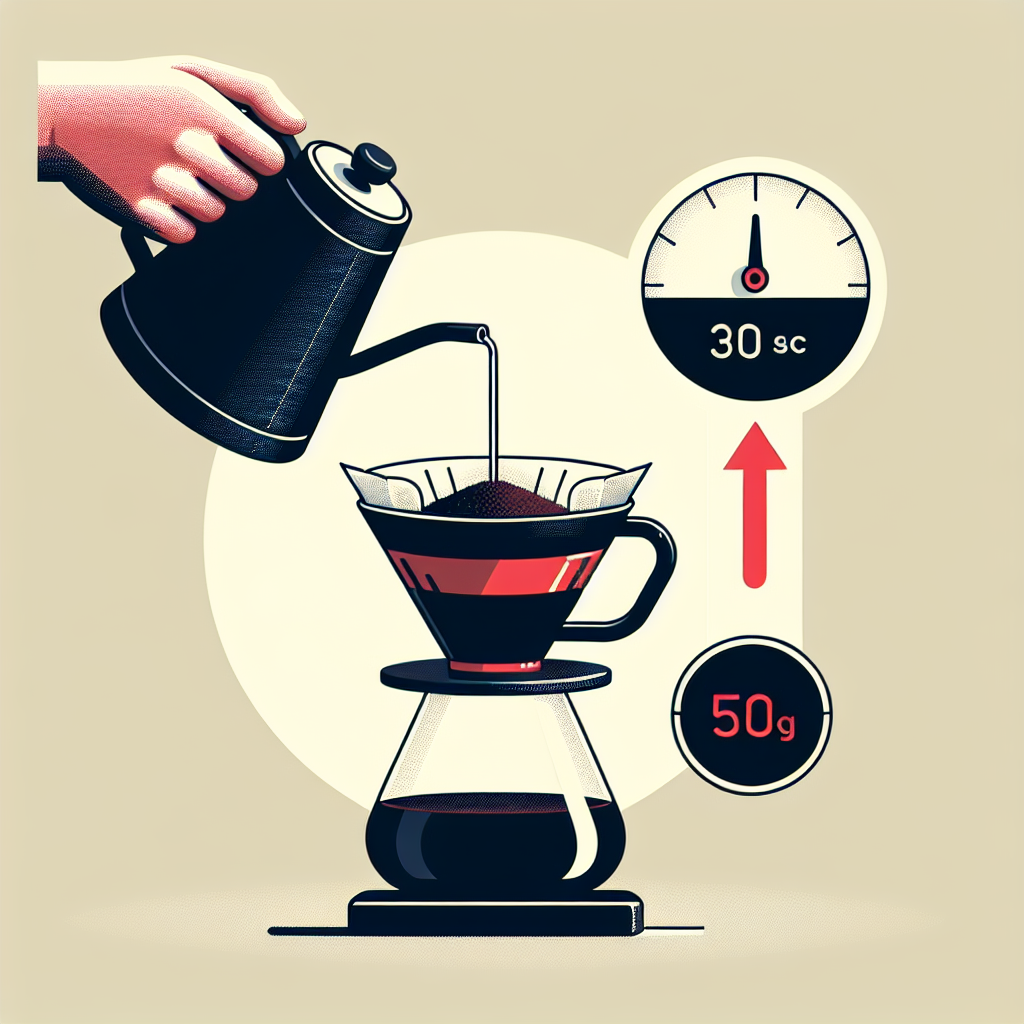}
        \caption{Set scale to zero}
        \label{fig:coffee-g}
    \end{subfigure}\hfill
    \caption{Steps for making pour-over coffee.}
    \label{fig:coffee}
\end{figure}

\subsection{Task4: Connect Switch to Monitor}
\paragraph{Prompt1: }Connect the black HDMI cable to the black HDMI port on the Nintendo Switch dock. Red arrow indicates the connection direction.

\paragraph{Prompt2: }connecting black type C power cable to the black dock of the Nintendo switch. Red arrow shows the connection direction.

\paragraph{Prompt3: }connecting black power cable to an AC outlet. Red arrow shows the direction of connection.

\paragraph{Prompt4: }Inserting Nintendo Switch into black Nintendo Switch dock. Red arrow shows direction of insertion.

\paragraph{Prompt5: }Press the power button on the Nintendo Switch console to turn it on. Red arrow indicates the power button location.

\paragraph{Prompt6: }black monitor with a visible power button in the left corner. pressing power button on monitor to turn it on. Red arrow indicates the power button location.

\begin{figure}[h]
    \centering
    \begin{subfigure}{0.16\textwidth}
        \centering
        \includegraphics[width=\textwidth]{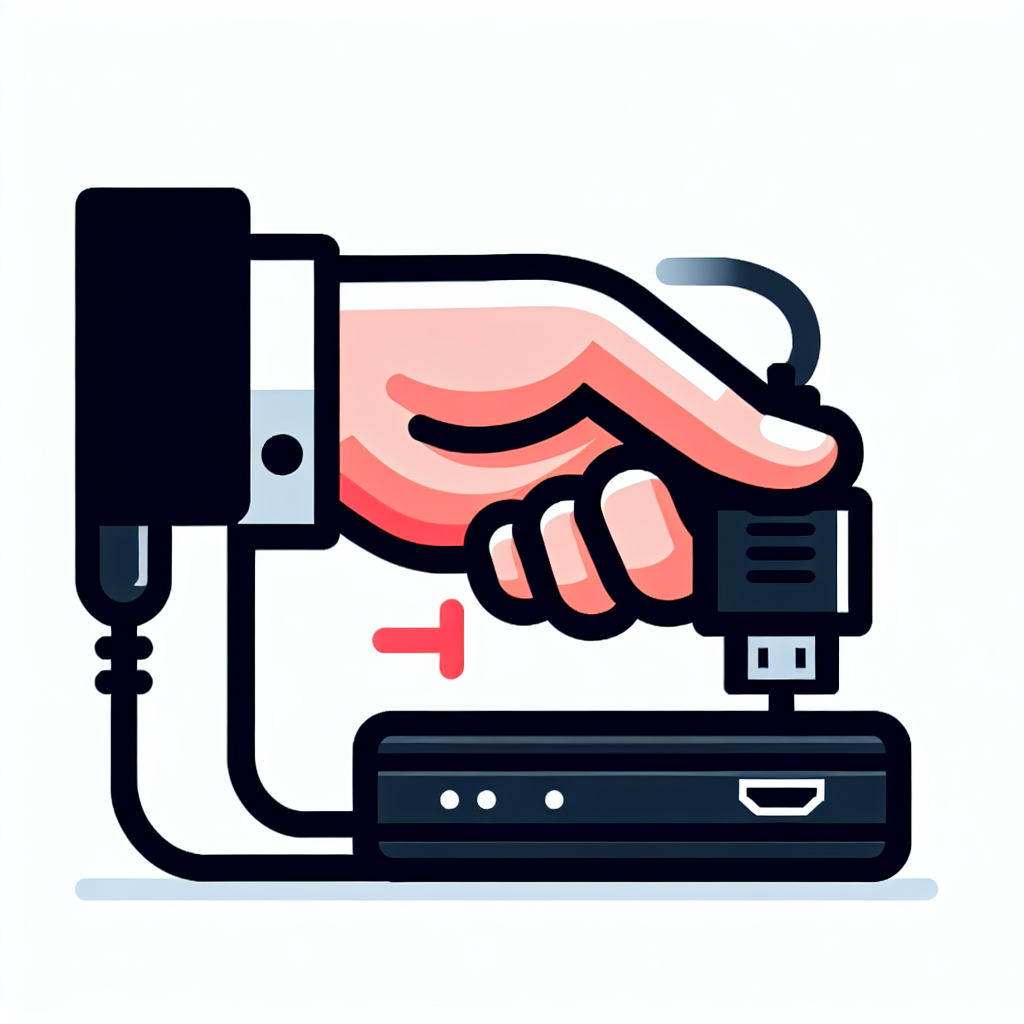}
        \caption{Connect HDMI cable}
        \label{fig:switch-a}
    \end{subfigure}\hfill
    \begin{subfigure}{0.16\textwidth}
        \centering
        \includegraphics[width=\textwidth]{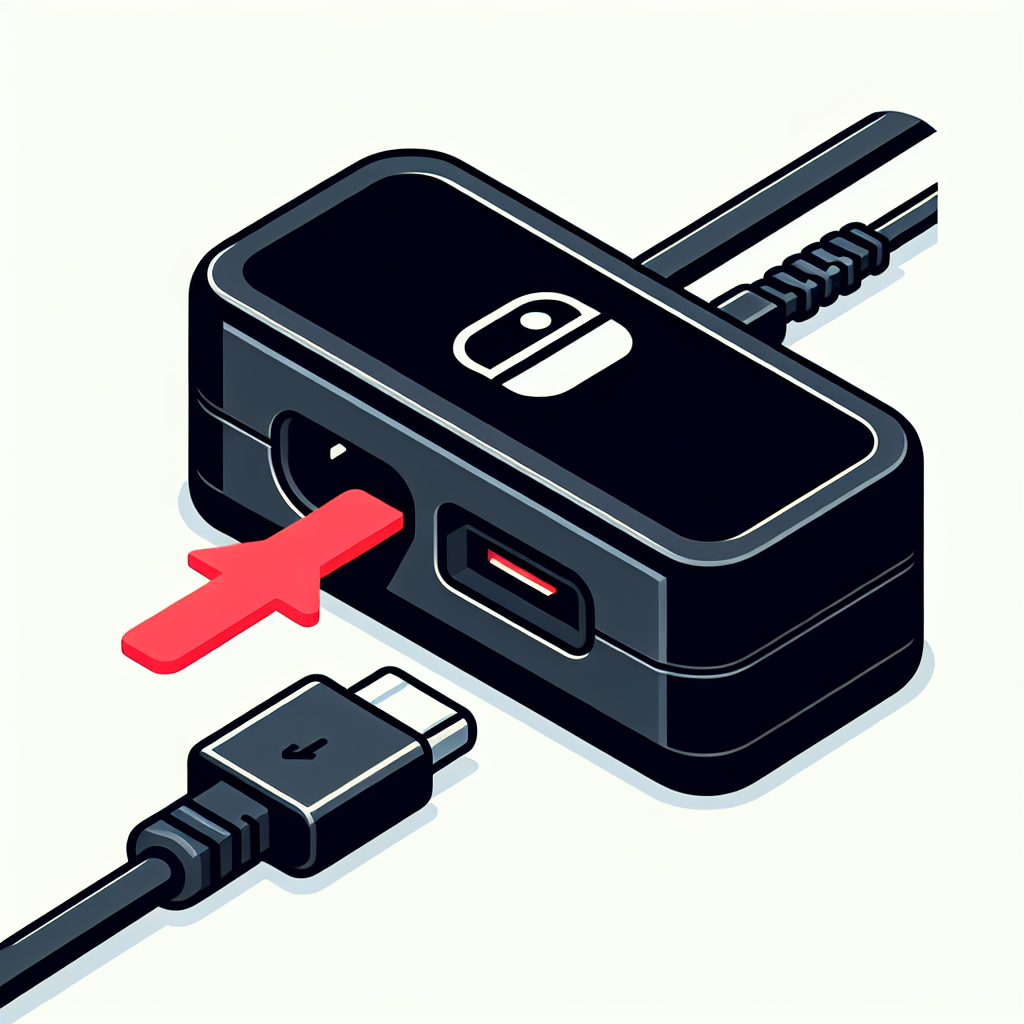}
        \caption{Connect Type C cable}
        \label{fig:switch-b}
    \end{subfigure}\hfill
    \begin{subfigure}{0.16\textwidth}
        \centering
        \includegraphics[width=\textwidth]{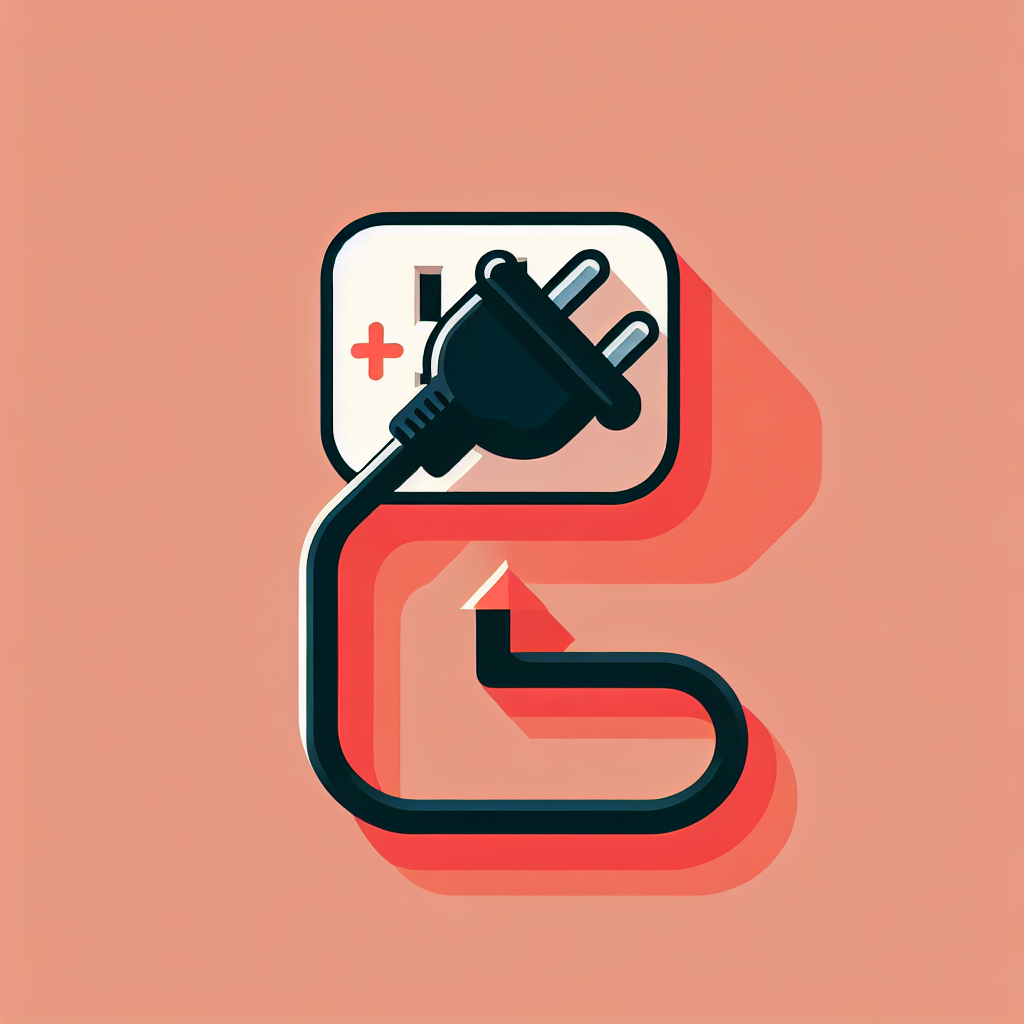}
        \caption{Connect power cable}
        \label{fig:switch-c}
    \end{subfigure}\hfill
    \begin{subfigure}{0.16\textwidth}
        \centering
        \includegraphics[width=\textwidth]{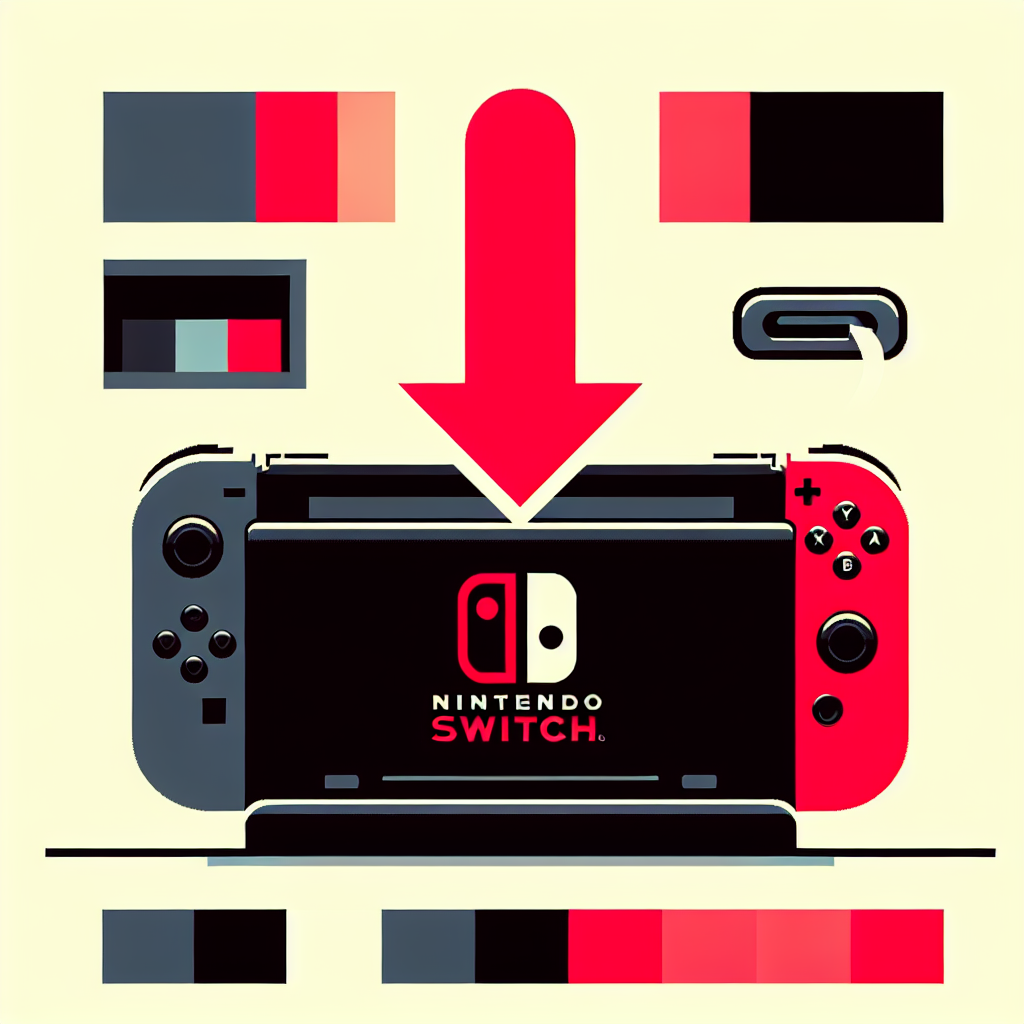}
        \caption{Insert Switch into dock}
        \label{fig:switch-d}
    \end{subfigure}\hfill
    \begin{subfigure}{0.16\textwidth}
        \centering
        \includegraphics[width=\textwidth]{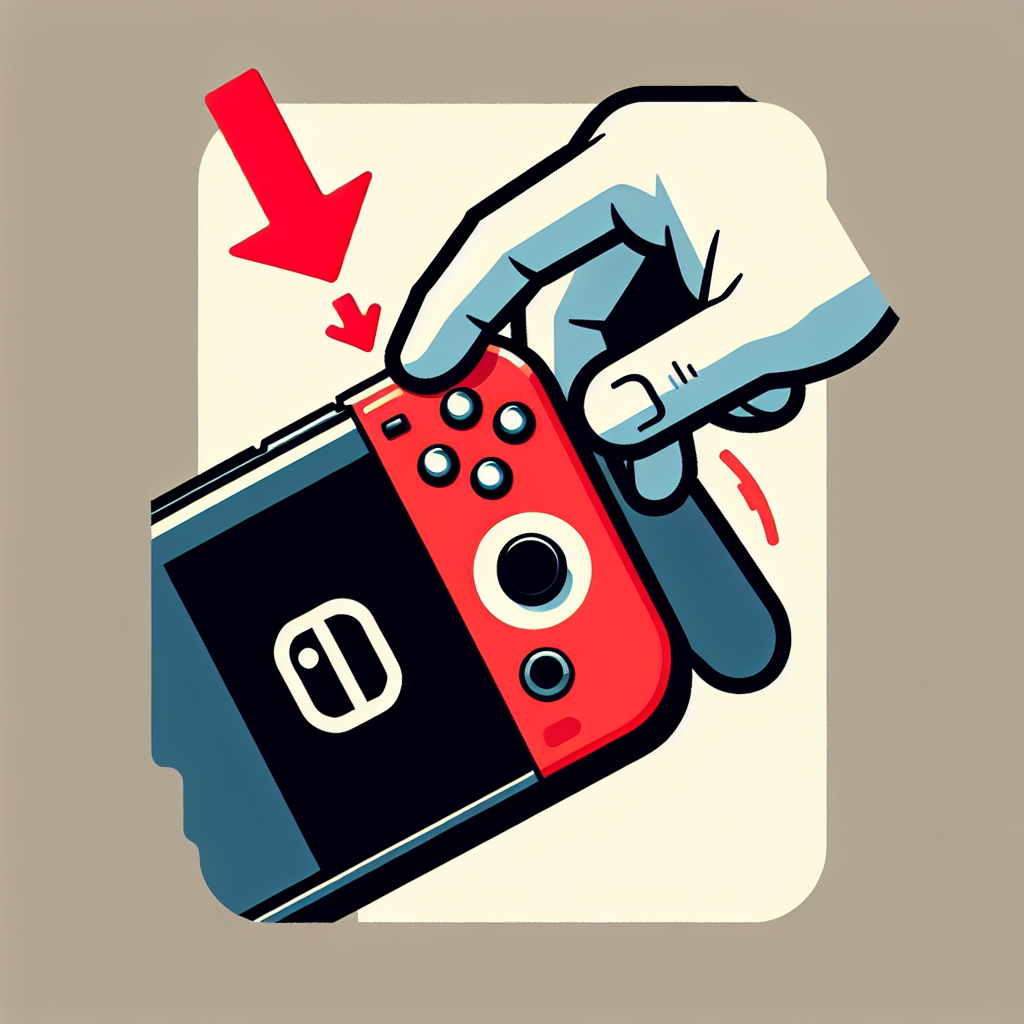}
        \caption{Press Switch power button}
        \label{fig:switch-e}
    \end{subfigure}\hfill
    \begin{subfigure}{0.16\textwidth}
        \centering
        \includegraphics[width=\textwidth]{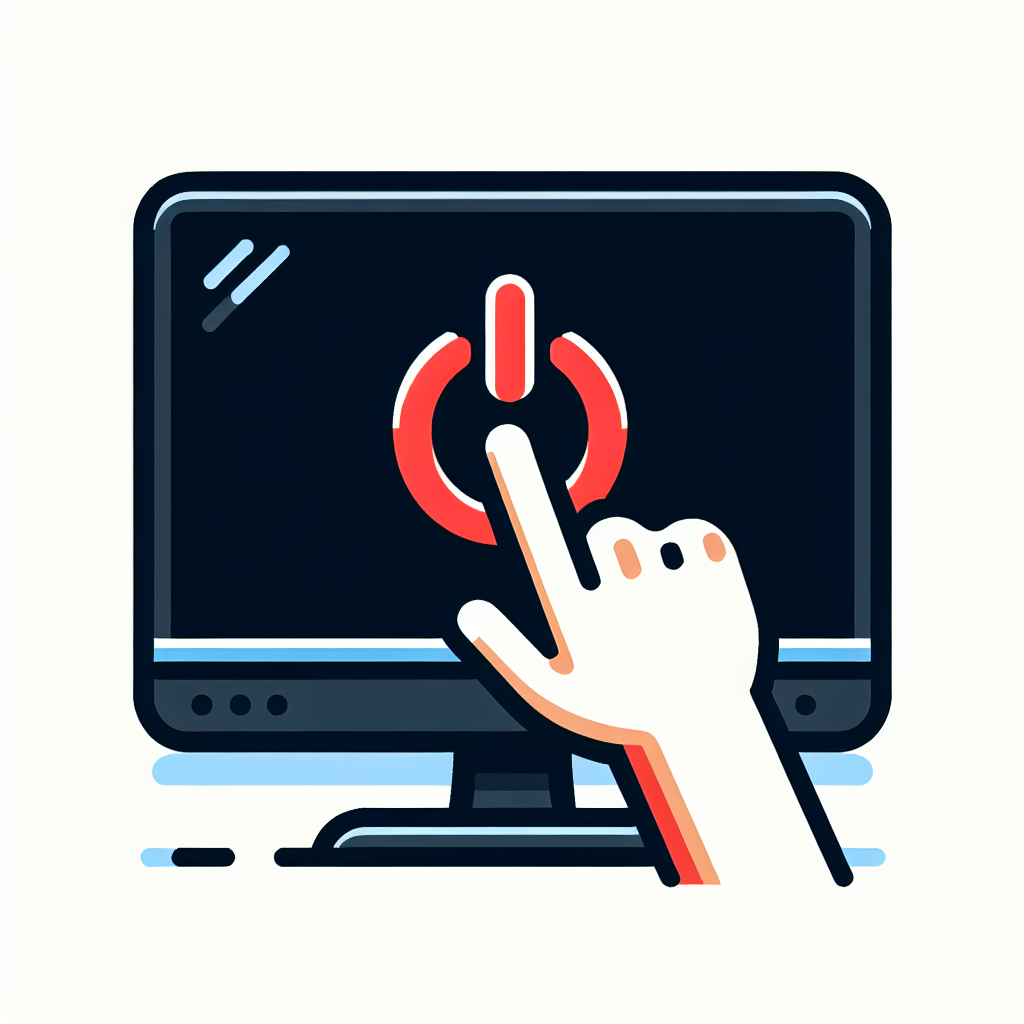}
        \caption{Turn on computer monitor}
        \label{fig:switch-f}
    \end{subfigure}
    \caption{Steps for connecting the Nintendo Switch to a monitor.}
    \label{fig:switch}
\end{figure}

\subsection{Comparison between original prompt and modified prompt}

As stated in Sec.\ref{dalle:comparison}, we present two examples of image assistance generation to demonstrate the effectiveness of our template, as shown Fig.\ref{fig:comparison}. 

The first example involves the task of making coffee. The basic prompt, without any modifier, is \participantquote{presses a button on an espresso machine.} Our enhanced prompt incorporates specific modifiers for clarity: \participantquote{presses a white button on a white espresso machine. A red arrow points to the button. No background, styled in flat, instructional illustrations. Accurate, concise, comfortable color style.}

In the second scenario, the user needs to cut the stem of a flower at a specific angle. The raw prompt reads: \participantquote{cuts stem of a flower up from the bottom with scissors at 45 degrees.} Our proposed prompt, enriched with detailed modifiers, is \participantquote{One hand cuts the stem of a red flower up from the bottom with white scissors at 45 degrees. A large red arrow points to the cut, set against a white background in the style of flat, instructional illustrations. Accurate, concise, comfortable color style.}

As shown in Fig ~\ref{fig:comparison}, Fig ~\ref{fig:comparison-a} and Fig ~\ref{fig:comparison-c}, derived from our template, eliminate unnecessary details and emphasize the core action of pressing a button. Clear visual elements, such as bold outlines and directional arrows, highlight the instructed action, making it immediately apparent what action is being instructed. This type of imagery is especially effective in instructional materials where rapid comprehension is essential. In contrast, Fig ~\ref{fig:comparison-b} and Fig ~\ref{fig:comparison-d} may introduce ambiguity in an instructional context due to their realistic depiction that includes reflective surfaces and shadows. While aesthetically pleasing, this level of detail can distract from the core instructional message. Therefore, our template enhances image clarity and directly aligns with the user’s need for clear, actionable instructions in their specific context.
