# Supplementary material for: Satori: Towards Proactive AR Assistant with Belief-Desire-Intention User Modeling
Source: arXiv:2410.16668 source file (2025-03-31)
Supplement: Supplementary file 3 [file 03_interview.tex]

\section{User Study Interview Quote}
We clustered the opinions shared by participants and presented the corresponding quotes. The opinions were collected through transcriptions of in-person interviews conducted after the experiments and from follow-up questionnaires.

\subsection{\systemname~System}

\subsubsection{Satori system is better for novice users} 
P8: \participantquote{if someone is new to, let's say, doing a certain task, there were visual cues that were there, which we had to see on the screen and replicate that.}

P6: \participantquote{if someone who doesn't know what is a grinder, or doesn't know what is the brewer, or stuff like that, it (animation) actually showed me.}

\subsubsection{Satori system can provide clear and useful instructions}

P8: \participantquote{though the tasks were simple, the instructions were very clear in both the things.}

P14: \participantquote{The guidance helps me a lot, especially in coffee making. It provides me with very detailed instructions including time, and amount of coffee beans I need. I would have to google it if I don't have the guidance.}
\subsubsection{Satori system can detect my intentions}

P9: \participantquote{the provided guidance pretty much aligned with my intention all the time. The confirmation message helps but also annoyed me a bit since it showed up after every step.}

P12: \participantquote{In my experience, most of the time the system knows what I have done in the past step eventually, but I wish it could be more responsive so I don't need to wait for the system to recognize what I have done}

\subsubsection{Design in Satori makes the users more engaged and feel trustworthy}
P9: \participantquote{I like to have a voice talking to me more for emotional support such as compliments after completing one step successfully. }
P5: \participantquote{The automatic step-by-step experience is highly engaging and makes me excited about its future. It gives me the impression that the machine understands what I'm doing, making its instructions feel trustworthy.}
P10: \participantquote{It automatically detects my progress.}
P12: \participantquote{I like how the system automatic play the text that you finished the task which made me more engaged at the beginning, but awhen I realize that it often takes time for the system to know you have finished and I have to wait for it, that engagement and enthusiasm faded.}

\subsubsection{Satori system can not always detect the completion of a step}

P8: \participantquote{most of the time…if I have to associate a number with it, 60\% of the time… it wasn't able to pick if I did finish the task or not.}

\subsubsection{Satori is bit lag behind Woz in terms of timely assistance}

P4: \participantquote{It was a bit delayed compared to the second one.}

P6: \participantquote{(Satori) I think maybe it took a little bit extra. I think five, 10 seconds extra I needed to show the image properly for it to understand that I've done the stuff. The second one, (WOZ) I saw that it could comprehend much more easily.}

\subsubsection{Satori main frustration point is detection of finish}

P3: \participantquote{But also I think that it would be helpful if it actually did recognize all of the things that I was doing.}

P2: \participantquote{the first system, what I feel is the guidance was good. The images were nice, the animation was on point, just the detection was not good.}

P9: \participantquote{I just hope the detection, whatever algorithm, can be more accurate, so I don't need to click it by myself.}

\subsubsection{The substep checkpoint and steps are useful}

P9: \participantquote{I like the mission kind of point of view, and it shows each step, like the sub-steps, with the progress checkings, like the circle thing. It's easier for me to understand if I'm working on the correct step, or if I already messed something up before I even noticed.}

P13: \participantquote{what you are doing and the overall objectives and individual steps. To show, like, it's easy to understand what step I did and going back and forth.}

\subsubsection{Combination of visual, text and audio modality makes task completion easier}

P3: \participantquote{So I like that the second system (SATORI) has also like a text feedback. So in case I'm lost, I can just figure it out. I think this one (WOZ) did not have a text feedback. So once I miss the voice, if I happen to miss the voice or if I forget, if it's a long task, then I might forget exactly where I am or what the subtasks involved in this task are.}

P3: \participantquote{Animations are helpful in either case. But the second one seems kind of more detailed. But I just feel that might be just because it combines different modalities. That I feel like better, a better sense of where I am in the task.}

P5: \participantquote{like, the images and the text and audio..the whole thing is composed more neatly.}

\subsubsection{Image assistance is useful}

P1: \participantquote{the picture of the second one is very nice and it looks good.}

P2: \participantquote{The images were nice, the animation was on point.}

P6: \participantquote{what I liked better was there was animation for everything. So yeah, I mean, if someone who doesn't know what is a grinder, or doesn't know what is the brewer, or stuff like that, it actually showed me. And who doesn't know how to cut below the waterline and stuff like that, it actually showed me the animation on whether to cut.}

\subsubsection{Image assistance is confusing, or complex}

P1: \participantquote{but I think it can be more simple because maybe many content in the picture is not necessary for me. icon can be just show the most important thing during the task and not many extra lines or something.}

P5: \participantquote{But in the second system, you just use, like, the AI-generated images. And that sometimes is just not, like, matching the real setting. So, sometimes if you use the real live objects, it may make the image instruction more clear.}

P14: \participantquote{sometimes the figure is confusing, I think because it's in flash style and it's sometimes it's a little different from what the actual item is.}

\subsubsection{Timer is useful}
P13: \participantquote{...for example the system gives video instructions on how to fold the coffee filter and place it in the cone; that's very helpful. I also like the timer when I make the coffee}
\subsubsection{Satori system gives user higher satisfaction on the assistance}

P2: \participantquote{I felt the first one was much better, but the second was, I felt I was able to do the task much faster. Reason: the first system, what I feel is the guidance was good. The images were nice, the animation was on point, just the detection was not good.}

\subsubsection{Task transitions are natural for both}

P2: \participantquote{in the two systems is it (natural). I felt there was a lag in first, in system one, but in system two, it was everything was robust.}

\subsubsection{Satori can be applied in daily life}
P12: \participantquote{I think this specific scenario is actually pretty helpful because sometimes we need to connect different devices that are new to us. I had a similar issue with my Wi-Fi router and modem at my apartment last year and I have to call a specialist to come and fix it, but an AR tutorial will be helpful.}

P8: \participantquote{Things like IKEA assembly etc., would be a great use case.}

P13: \participantquote{cooking, assembling equipment (ex. PC) or furnitures (ex. shelf), operating on machines (ex. coffee maker), exercise (ex. different yoga moves)}

P9: \participantquote{...maybe when we need to assembly a furniture, instead of going through the manual back and forth all the time, we can just have this system to guide us.}

\subsection{\baseline~}

\subsubsection{\baseline~system detect user's intentions}
P9: \participantquote{There is no misalignment between my intentions and the provided guidance}

P13: \participantquote{sometimes there are time lag, but mostly it works fine}

\subsubsection{The modality design is not as much as helpful}

P1: \participantquote{The timing of the first one is really not useful for me because I cannot figure out whether which way it will present to me. Maybe the voice, maybe the image. There was a time that I think it will be a voice to lead me but actually there is an image but I didn't know. I just wait for the voice and I don't know how to do the next.}

P2: \participantquote{...However, the lack of text guidance made some tasks more difficult.}

P4: \participantquote{Its guidance was not uniform. It showed text, audio, images randomly. When I need a animation to help, it only showed me a text.}

\subsubsection{Woz helps user complete the task faster and smoother}

P2: \participantquote{I felt the first one was much better, but the second was, I felt I was able to do the task much faster. I would definitely prefer like the system two, over like system one, because it's much faster, even though there are less instructions (WOZ).}

P8: \participantquote{This system had through-and-through audio guidance. This helped me feel the process was much smoother}

P2: \participantquote{The guidance in System B was helpful due to the fast detection of task completion. For example, when connecting the mop and duster, the system quickly recognized the task as complete. }

\subsubsection{Animation and image assistance are better}

P9: \participantquote{animation from the last one, from the first system, was easier to follow compared to the images that's in today's system.}

\participantquote{The system gives me realistic images and voice guidance.}
